# Supplementary material for: Magnon Interference Tunneling Spectroscopy as a Probe of 2D Magnetism
Source: arXiv:2110.02662 source file (2021-10-06)
Supplement: Supplementary file 1 [file Magnon_QPI_SM.pdf]

# *Supplementary Material*: Magnon Interference Tunneling Spectroscopy as a Probe of 2D Magnetism

Asimpunya Mitra,[1] Alberto Corticelli,[2] Pedro Ribeiro,[3,4] and Paul A. McClarty[2]

[1]*Indian Institute of Technology Kharagpur, Kharagpur 721302, India*
[2]*Max Planck Institute for the Physics of Complex Systems, Nöthnitzer Str. 38, 01187 Dresden, Germany*
[3]*CeFEMA, Instituto Superior Técnico, Universidade de Lisboa, Av. Rovisco Pais, 1049-001 Lisboa, Portugal*
[4]*Beijing Computational Science Research Center, Beijing 100084, China*

This Supplementary Material provides additional technical details: (1) a detailed calculation of the tunneling current, (2) a calculation of the inelastic tunneling contribution including a brief introduction to spin wave theory and definitions of the various spin models we consider in the paper, (3) results for the magnon contribution to single site tunneling in a lattice without disorder, (4) a detailed discussion of the methods used to compute the local dynamical structure factor for magnons in the presence of an impurity as well as extensive results for the local dynamical structure factor in the presence of a vacancy, (5) further results on topological magnons.

## 1. TUNNELING CURRENT

### 1.1. Overview

We consider a conducting substrate with a magnetic layer deposited onto it and a metallic STM tip which can be moved around above the magnetic layer. A voltage of $V$ is applied between the conducting substrate and the tip. The presence of the magnetic layer enables two types of tunneling processes between the tip and the substrate: elastic tunneling processes - exchange of electrons between tip and substrate without interacting with the magnetic layer, inelastic tunneling processes - exchange of electrons between the tip and the substrate mediated by an interaction with the magnetic layer. We consider the magnetic layer to be a weakly hybridised Anderson impurity model which supports local moment formation. This model is renormalised to expose its low-energy structure, which is then used to calculate the tunneling current within linear response theory.

Our primary interest is in the inelastic tunneling processes as these contain information regarding the magnetic layer. The elastic tunneling current is Ohmic while the inelastic tunneling current is non-Ohmic. Thus the inelastic tunneling conductance has a non-trivial voltage dependence, and this dependence is used to extract some properties of the magnon excitations in these 2D magnetic systems.

While our discussion is self-contained, there is a considerable relevant literature. We refer to a small cross-section that has some reasonably direct bearing on the derivation given below (see, for example, [1–6]).

### 1.2. Calculation of Tunneling Conductance with Magnetic Scattering

We suppose the metallic tip is at lateral position $\boldsymbol{r}_{\rm T}$ and the Hamiltonian of the tip is $H_{\rm tip} = \sum_{\mathbf{k}\sigma} \epsilon_{\rm T\mathbf{k}} f^{\dagger}_{\mathbf{k}\sigma} f_{\mathbf{k}\sigma}$. The substrate is a $2D$ lattice with sites at $\boldsymbol{r}_{\rm S}$ and Hamiltonian $H_{\rm sub} = \sum_{\mathbf{k}\sigma} \epsilon_{\rm S\mathbf{k}} c^{\dagger}_{\mathbf{k}\sigma} c_{\mathbf{k}\sigma}$. The temperature is set to zero and, in practice, it is important to work at temperatures much smaller than the exchange scale in the magnetic layer. The magnetic layer is treated as an Anderson impurity model which consists of a $2D$ lattice of impurity sites denoted by $d^{\dagger}_{\boldsymbol{r}_{\rm I}\sigma}$. The vertical distance between the STM tip and the magnetic layer is $d_1$ and that between the magnetic layer and the substrate is $d_2$. The presence of a large Coulomb barrier inhibits double occupancy of the impurity sites. A spin conserving coupling between the impurity level and the metallic tips and substrate lead to hybridization of the states. The tunneling amplitude from the tip to the magnetic layer is $t_1(\boldsymbol{r}_{\rm T} - \boldsymbol{r}_{\rm I})$, and from the magnetic layer to the substrate is $t_2(\boldsymbol{r}_{\rm I} - \boldsymbol{r}_{\rm S})$. Additionally intra-layer hoppings $H_{\rm mag}$ are present in the impurity layer which give rise to magnetic ordering in this layer. The total Hamiltonian of the system is

$$
\begin{aligned}
H = &\sum_{\mathbf{k}\sigma} \epsilon_{\rm S\mathbf{k}} c^{\dagger}_{\mathbf{k}\sigma} c_{\mathbf{k}\sigma} + \sum_{\mathbf{k}\sigma} \epsilon_{\rm T\mathbf{k}} f^{\dagger}_{\mathbf{k}\sigma} f_{\mathbf{k}\sigma} + \sum_{\boldsymbol{r}_{\rm I}\sigma} \epsilon_d d^{\dagger}_{\boldsymbol{r}_{\rm I}\sigma} d_{\boldsymbol{r}_{\rm I}\sigma} + \sum_{\boldsymbol{r}_{\rm I}} U n_{d\boldsymbol{r}_{\rm I}\uparrow} n_{d\boldsymbol{r}_{\rm I}\downarrow} \\
&+ \sum_{\boldsymbol{r}_{\rm I}\sigma} d^{\dagger}_{\boldsymbol{r}_{\rm I}\sigma} \left( t_1(\boldsymbol{r}_{\rm T} - \boldsymbol{r}_{\rm I}) f_{\boldsymbol{r}_{\rm T}\sigma} + \sum_{\boldsymbol{r}_{\rm S}} t_2(\boldsymbol{r}_{\rm I} - \boldsymbol{r}_{\rm S}) c_{\boldsymbol{r}_{\rm S}\sigma} \right) + \text{h.c.} + H_{\rm mag}.
\end{aligned} \tag{1.1}
$$

At low energies the model has single occupancy in the magnetic layer with its integrity protected by large Hubbard-$U$ Coulomb interactions, and in the limit of $U \gg \epsilon_d \gg \Delta_{hyb}$ this model supports local moment formation. The effective low energy limit of the Hamiltonian is then realised as a perturbation over the singly occupied Hubbard system. We express the total wavefunction $|\psi\rangle$ as a sum of $|\psi_1\rangle$, $|\psi_2\rangle$, $|\psi_3\rangle$ where the index denotes the occupancy of the impurity site. The Schrodinger equation is rearranged as

$\hat{H}_{mn}\left|\psi_n\right\rangle = E\left|\psi_n\right\rangle$, where $\hat{H}_{mn} = \hat{P}_m \hat{H} \hat{P}_n$ and $\hat{P}_m$ are projectors onto the subspace with $m$ electrons. Then $\left|\psi_1\right\rangle$ is the wavefunction for the singly occupied impurity sites and using perturbation theory

$$\left(H_{10}\frac{1}{E-H_{00}}H_{01} + H_{12}\frac{1}{E-H_{22}}H_{21} + H_{11}\right)\left|\psi_1\right\rangle = E\left|\psi_1\right\rangle \tag{1.2}$$

$$H_{11} = \sum_{\mathbf{k}\sigma}\epsilon_{\mathrm{S}\mathbf{k}} c^\dagger_{\mathbf{k}\sigma}c_{\mathbf{k}\sigma} + \sum_{\mathbf{k}\sigma}\epsilon_{\mathrm{T}\mathbf{k}} f^\dagger_{\mathbf{k}\sigma}f_{\mathbf{k}\sigma} + N\epsilon_d \tag{1.3}$$

$$H_{10} = \sum_{\boldsymbol{r}_\mathrm{I}\sigma} d^\dagger_{\boldsymbol{r}_\mathrm{I}\sigma}(1 - n_{d_{r_\mathrm{I}}\bar{\sigma}})\left(t_1(\boldsymbol{r}_\mathrm{T}-\boldsymbol{r}_\mathrm{I})f_{\boldsymbol{r}_\mathrm{T}\sigma} + \sum_{\boldsymbol{r}_\mathrm{S}} t_2(\boldsymbol{r}_\mathrm{I}-\boldsymbol{r}_\mathrm{S})c_{\boldsymbol{r}_\mathrm{S}\sigma}\right) \tag{1.4}$$

$$H_{21} = \sum_{\boldsymbol{r}_\mathrm{I}\sigma} d^\dagger_{\boldsymbol{r}_\mathrm{I}\sigma} n_{d_{r_\mathrm{I}}\bar{\sigma}}\left(t_1(\boldsymbol{r}_\mathrm{T}-\boldsymbol{r}_\mathrm{I})f_{\boldsymbol{r}_\mathrm{T}\sigma} + \sum_{\boldsymbol{r}_\mathrm{S}} t_2(\boldsymbol{r}_\mathrm{I}-\boldsymbol{r}_\mathrm{S})c_{\boldsymbol{r}_\mathrm{S}\sigma}\right) \tag{1.5}$$

$$H_{01} = H^\dagger_{10} \qquad H_{12} = H^\dagger_{21}. \tag{1.6}$$

The energy obtained from perturbation theory above is expanded to leading order in $1/U$ and $1/\epsilon_d$. This gives a renormalised low energy Hamiltonian of the form $H = H_0 + \delta H$, where $H_0$ has terms which describe the unperturbed tip or substrate or magnetic layer, and $\delta H$ has terms which, among other things, contribute to the tunneling between the layers by exchange of fermions [7]:

$$H_0 = \sum_{\mathbf{k}\sigma}\epsilon_{\mathrm{S}\mathbf{k}} c^\dagger_{\mathbf{k}\sigma}c_{\mathbf{k}\sigma} + \sum_{\mathbf{k}\sigma}\epsilon_{\mathrm{T}\mathbf{k}} f^\dagger_{\mathbf{k}\sigma}f_{\mathbf{k}\sigma} + N\epsilon_d + \frac{1}{\epsilon_d}\sum_{\boldsymbol{r}_\mathrm{I}\boldsymbol{r}'_\mathrm{I}\sigma}\left(t^*_1(\boldsymbol{r}_\mathrm{T}-\boldsymbol{r}_\mathrm{I})t_1(\boldsymbol{r}_\mathrm{T}-\boldsymbol{r}'_\mathrm{I}) + \sum_{\boldsymbol{r}_\mathrm{S}} t^*_2(\boldsymbol{r}_\mathrm{I}-\boldsymbol{r}_\mathrm{S})t_2(\boldsymbol{r}'_\mathrm{I}-\boldsymbol{r}_\mathrm{S})\right)d^\dagger_{\boldsymbol{r}'_\mathrm{I}\sigma}d_{\boldsymbol{r}_\mathrm{I}\sigma} \tag{1.7}$$

$$\begin{aligned}
\delta H = &\left(\frac{1}{U+\epsilon_d} - \frac{1}{\epsilon_d}\right)\left(\sum_{\boldsymbol{r}_\mathrm{I}\boldsymbol{r}'_\mathrm{I}\boldsymbol{r}_\mathrm{S}} t^*_1(\boldsymbol{r}_\mathrm{T}-\boldsymbol{r}_\mathrm{I})t_2(\boldsymbol{r}'_\mathrm{I}-\boldsymbol{r}_\mathrm{S})\left(\sum_{\alpha\beta} f^\dagger_{\boldsymbol{r}_\mathrm{T}\alpha}\sigma_{\alpha\beta}c_{\boldsymbol{r}_\mathrm{S}\beta}\right)\cdot\left(\frac{1}{2}\sum_{\gamma\delta} d^\dagger_{\boldsymbol{r}'_\mathrm{I}\gamma}\sigma_{\gamma\delta}d_{\boldsymbol{r}_\mathrm{I}\delta}\right) + \text{h.c.}\right)\\
&+\left(\frac{1}{U+\epsilon_d} - \frac{1}{\epsilon_d}\right)\sum_{\boldsymbol{r}_\mathrm{I}\boldsymbol{r}'_\mathrm{I}} t^*_1(\boldsymbol{r}_\mathrm{T}-\boldsymbol{r}_\mathrm{I})t_1(\boldsymbol{r}_\mathrm{T}-\boldsymbol{r}'_\mathrm{I})\left(\sum_{\alpha\beta} f^\dagger_{\boldsymbol{r}_\mathrm{T}\alpha}\sigma_{\alpha\beta}f_{\boldsymbol{r}_\mathrm{T}\beta}\right)\cdot\left(\frac{1}{2}\sum_{\gamma\delta} d^\dagger_{\boldsymbol{r}'_\mathrm{I}\gamma}\sigma_{\gamma\delta}d_{\boldsymbol{r}_\mathrm{I}\delta}\right)\\
&+\left(\frac{1}{U+\epsilon_d} - \frac{1}{\epsilon_d}\right)\sum_{\boldsymbol{r}_\mathrm{I}\boldsymbol{r}'_\mathrm{I}\boldsymbol{r}_\mathrm{S}\boldsymbol{r}'_\mathrm{S}} t^*_2(\boldsymbol{r}_\mathrm{I}-\boldsymbol{r}'_\mathrm{S})t_2(\boldsymbol{r}'_\mathrm{I}-\boldsymbol{r}_\mathrm{S})\left(\sum_{\alpha\beta} c^\dagger_{\boldsymbol{r}'_\mathrm{S}\alpha}\sigma_{\alpha\beta}c_{\boldsymbol{r}_\mathrm{S}\beta}\right)\cdot\left(\frac{1}{2}\sum_{\gamma\delta} d^\dagger_{\boldsymbol{r}'_\mathrm{I}\gamma}\sigma_{\gamma\delta}d_{\boldsymbol{r}_\mathrm{I}\delta}\right)\\
&-\left(\frac{1}{U+\epsilon_d}\right)\sum_{\boldsymbol{r}_\mathrm{I}\sigma}\left(|t_1(\boldsymbol{r}_\mathrm{T}-\boldsymbol{r}_\mathrm{I})|^2 f^\dagger_{\boldsymbol{r}_\mathrm{T}\sigma}f_{\boldsymbol{r}_\mathrm{T}\sigma} + \sum_{\boldsymbol{r}_\mathrm{S}\boldsymbol{r}'_\mathrm{S}} t^*_2(\boldsymbol{r}_\mathrm{I}-\boldsymbol{r}'_\mathrm{S})t_2(\boldsymbol{r}_\mathrm{I}-\boldsymbol{r}_\mathrm{S})c^\dagger_{\boldsymbol{r}'_\mathrm{S}\sigma}c_{\boldsymbol{r}_\mathrm{S}\sigma}\right) - \left(\frac{1}{U+\epsilon_d}\right)\left(\sum_{\boldsymbol{r}_\mathrm{I}\boldsymbol{r}_\mathrm{S}\sigma} t^*_1(\boldsymbol{r}_\mathrm{T}-\boldsymbol{r}_\mathrm{I})t_2(\boldsymbol{r}_\mathrm{I}-\boldsymbol{r}_\mathrm{S})f^\dagger_{\boldsymbol{r}_\mathrm{T}\sigma}c_{\boldsymbol{r}_\mathrm{S}\sigma} + \text{h.c.}\right)\\
&+\frac{1}{2}\left(\frac{1}{U+\epsilon_d} - \frac{1}{\epsilon_d}\right)\sum_{\boldsymbol{r}_\mathrm{I}\boldsymbol{r}'_\mathrm{I}\sigma\sigma'}\left(t^*_1(\boldsymbol{r}_\mathrm{T}-\boldsymbol{r}_\mathrm{I})t_1(\boldsymbol{r}_\mathrm{T}-\boldsymbol{r}'_\mathrm{I})f^\dagger_{\boldsymbol{r}_\mathrm{T}\sigma}f_{\boldsymbol{r}_\mathrm{T}\sigma} + \sum_{\boldsymbol{r}_\mathrm{S}\boldsymbol{r}'_\mathrm{S}} t^*_2(\boldsymbol{r}_\mathrm{I}-\boldsymbol{r}'_\mathrm{S})t_2(\boldsymbol{r}'_\mathrm{I}-\boldsymbol{r}_\mathrm{S})c^\dagger_{\boldsymbol{r}'_\mathrm{S}\sigma}c_{\boldsymbol{r}_\mathrm{S}\sigma}\right)d^\dagger_{\boldsymbol{r}'_\mathrm{I}\sigma'}d_{\boldsymbol{r}_\mathrm{I}\sigma'}\\
&+\frac{1}{2}\left(\frac{1}{U+\epsilon_d} - \frac{1}{\epsilon_d}\right)\left(\sum_{\boldsymbol{r}_\mathrm{I}\boldsymbol{r}'_\mathrm{I}\boldsymbol{r}_\mathrm{S}\sigma\sigma'} t^*_1(\boldsymbol{r}_\mathrm{T}-\boldsymbol{r}_\mathrm{I})t_2(\boldsymbol{r}'_\mathrm{I}-\boldsymbol{r}_\mathrm{S})f^\dagger_{\boldsymbol{r}_\mathrm{T}\sigma}c_{\boldsymbol{r}_\mathrm{S}\sigma}d^\dagger_{\boldsymbol{r}'_\mathrm{I}\sigma'}d_{\boldsymbol{r}_\mathrm{I}\sigma'} + \text{h.c.}\right).
\end{aligned} \tag{1.8}$$

The first term of (1.8) can be rearranged to express it in terms of $\sum_{\boldsymbol{r}_\mathrm{I},\boldsymbol{r}'_\mathrm{I},\boldsymbol{r}_\mathrm{S}} J(\boldsymbol{r}_\mathrm{T}-\boldsymbol{r}_\mathrm{I},\boldsymbol{r}'_\mathrm{I}-\boldsymbol{r}_\mathrm{S})\boldsymbol{S}_{\boldsymbol{r}_\mathrm{I},\boldsymbol{r}'_\mathrm{I}}\cdot \boldsymbol{s}_{\boldsymbol{r}_\mathrm{T},\boldsymbol{r}_\mathrm{S}}$, where $S^i_{\boldsymbol{r}_\mathrm{I},\boldsymbol{r}'_\mathrm{I}} = d^\dagger_{\boldsymbol{r}_\mathrm{I},s}\sigma^i_{s,s'}d_{\boldsymbol{r}'_\mathrm{I},s'}$ and $s^i_{\boldsymbol{r}_\mathrm{T},\boldsymbol{r}_\mathrm{S}} = f^\dagger_{\boldsymbol{r}_\mathrm{T},s}\sigma^i_{s,s'}c_{\boldsymbol{r}_\mathrm{S},s'}$. Only this term will give a contribution to the inelastic tunneling current calculated in (1.20).

To calculate the tunneling current we use linear response theory, so the current is due to the presence of the perturbation $\delta H = T + T^\dagger$. The current operator is $I = e\frac{dN_{tip}}{dt} = \frac{e}{i\hbar}[N_{tip}, H] = J + J^\dagger$.

$$\begin{aligned}
T = &\left(\frac{1}{U+\epsilon_d} - \frac{1}{\epsilon_d}\right)\sum_{\boldsymbol{r}_\mathrm{I}\boldsymbol{r}'_\mathrm{I}\boldsymbol{r}_\mathrm{S}} t^*_1(\boldsymbol{r}_\mathrm{T}-\boldsymbol{r}_\mathrm{I})t_2(\boldsymbol{r}'_\mathrm{I}-\boldsymbol{r}_\mathrm{S})\left(\sum_{\alpha\beta} f^\dagger_{\boldsymbol{r}_\mathrm{T}\alpha}\sigma_{\alpha\beta}c_{\boldsymbol{r}_\mathrm{S}\beta}\right)\cdot\left(\frac{1}{2}\sum_{\gamma\delta} d^\dagger_{\boldsymbol{r}'_\mathrm{I}\gamma}\sigma_{\gamma\delta}d_{\boldsymbol{r}_\mathrm{I}\delta}\right)\\
&+\frac{1}{2}\left(\frac{1}{U+\epsilon_d} - \frac{1}{\epsilon_d}\right)\sum_{\boldsymbol{r}_\mathrm{I}\boldsymbol{r}'_\mathrm{I}\boldsymbol{r}_\mathrm{S}\sigma\sigma'} t^*_1(\boldsymbol{r}_\mathrm{T}-\boldsymbol{r}_\mathrm{I})t_2(\boldsymbol{r}'_\mathrm{I}-\boldsymbol{r}_\mathrm{S})f^\dagger_{\boldsymbol{r}_\mathrm{T}\sigma}c_{\boldsymbol{r}_\mathrm{S}\sigma}d^\dagger_{\boldsymbol{r}'_\mathrm{I}\sigma'}d_{\boldsymbol{r}_\mathrm{I}\sigma'} - \left(\frac{1}{U+\epsilon_d}\right)\sum_{\boldsymbol{r}_\mathrm{I}\boldsymbol{r}_\mathrm{S}\sigma} t^*_1(\boldsymbol{r}_\mathrm{T}-\boldsymbol{r}_\mathrm{I})t_2(\boldsymbol{r}_\mathrm{I}-\boldsymbol{r}_\mathrm{S})f^\dagger_{\boldsymbol{r}_\mathrm{T}\sigma}c_{\boldsymbol{r}_\mathrm{S}\sigma}
\end{aligned} \tag{1.9}$$

$$J=\frac{ie}{\hbar}\left(\frac{1}{U+\epsilon_d}-\frac{1}{\epsilon_d}\right)\sum_{r_{\rm I}r'_{\rm I}r_{\rm S}}t_1^*(r_{\rm T}-r_{\rm I})t_2(r'_{\rm I}-r_{\rm S})\left(\sum_{\alpha\beta}f^\dagger_{r_{\rm T}\alpha}\sigma_{\alpha\beta}c_{r_{\rm S}\beta}\right)\cdot\left(\frac{1}{2}\sum_{\gamma\delta}d^\dagger_{r'_{\rm I}\gamma}\sigma_{\gamma\delta}d_{r_{\rm I}\delta}\right)$$

$$+\frac{ie}{2\hbar}\left(\frac{1}{U+\epsilon_d}-\frac{1}{\epsilon_d}\right)\sum_{r_{\rm I}r'_{\rm I}r_{\rm S}\sigma\sigma'}t_1^*(r_{\rm T}-r_{\rm I})t_2(r'_{\rm I}-r_{\rm S})f^\dagger_{r_{\rm T}\sigma}c_{r_{\rm S}\sigma}d^\dagger_{r'_{\rm I}\sigma'}d_{r_{\rm I}\sigma'}-\frac{ie}{\hbar}\left(\frac{1}{U+\epsilon_d}-\frac{1}{\epsilon_d}\right)\sum_{r_{\rm I}r_{\rm S}\sigma}t_1^*(r_{\rm T}-r_{\rm I})t_2(r_{\rm I}-r_{\rm S})f^\dagger_{r_{\rm T}\sigma}c_{r_{\rm S}\sigma}. \quad (1.10)$$

Using (1.9), (1.10), the tunneling current is computed as

$$\langle I\rangle=\langle J\rangle+\left\langle J^\dagger\right\rangle=2\int_{-\infty}^{t}dt' Re[\chi_{JT^\dagger}(t-t')] \quad (1.11)$$

$$\chi_{JT^\dagger}(t-t')=-\frac{i}{\hbar}\Theta(t-t')\left\langle\left[J(t),T^\dagger(t')\right]\right\rangle_{eq} \quad (1.12)$$

where $\chi_{JT^\dagger}(t-t')$ is the retarded response function calculated in equilibrium.

The tunneling current has two contributions. One is from an elastic process − exchange from tip to substrate − and the other is from inelastic processes − exchange from tip to magnetic layer and again from magnetic layer to substrate. To compute the response function we use a momentum space representation of $J$ and $T^\dagger$.

The response function $\chi_{JT^\dagger}(t-t')$ can be written as a sum of an elastic response function $\chi_{1JT^\dagger}(t-t')$ and an inelastic response function $\chi_{2JT^\dagger}(t-t')$. Evaluating the response functions we find that

$$\chi_{1JT^\dagger}(t-t')=\frac{Ae\Theta(t-t')}{\hbar^2N^2}\sum_{r_{\rm I}r'_{\rm I}r_{\rm S}r'_{\rm S}kk'\sigma}t_1^*(r_{\rm I}-r_{\rm T})t_2(r_{\rm I}-r_{\rm S})t_1(r_{\rm T}-r'_{\rm I})t_2^*(r'_{\rm I}-r'_{\rm S})e^{i\mathbf{k}'\cdot(r_{\rm S}-r'_{\rm S})}\left(n_{T\mathbf{k}\sigma}-n_{S\mathbf{k}'\sigma}\right)e^{\frac{i(t-t')}{\hbar}(\epsilon_{T\mathbf{k}}-\epsilon_{S\mathbf{k}'})} \quad (1.13)$$

$$\chi_{2JT^\dagger}(t-t')=\frac{2Be\Theta(t-t')}{\hbar^2N^2}\sum_{r_{\rm I}r'_{\rm I}r_{\rm S}r'_{\rm S}kk'\alpha}t_1^*(r_{\rm I}-r_{\rm T})t_2(r_{\rm S}-r_{\rm I})t_1(r'_{\rm I}-r_{\rm T})t_2^*(r'_{\rm S}-r'_{\rm I})e^{i\mathbf{k}'\cdot(r_{\rm S}-r'_{\rm S})}e^{\frac{i(t-t')}{\hbar}(\epsilon_{T\mathbf{k}}-\epsilon_{S\mathbf{k}'})}$$

$$\left(n_{\rm T\mathbf{k}}(1-n_{\rm S\mathbf{k}'})\left\langle S^\alpha_{r_{\rm I}}(t)S^\alpha_{r'_{\rm I}}(t')\right\rangle-n_{\rm S\mathbf{k}'}(1-n_{\rm T\mathbf{k}})\left\langle S^\alpha_{r'_{\rm I}}(t')S^\alpha_{r_{\rm I}}(t)\right\rangle\right) \quad (1.14)$$

where $A=\frac{1}{4}\left(\frac{1}{U+\epsilon_d}+\frac{1}{\epsilon_d}\right)^2$ and $B=\left(\frac{1}{U+\epsilon_d}-\frac{1}{\epsilon_d}\right)^2$. The Fermi distributions for the tip and substrate at $T=0$ are $n_{\rm T\mathbf{k}\sigma}=\langle f^\dagger_{\mathbf{k}\sigma}f_{\mathbf{k}\sigma}\rangle_{T=0}=\Theta(\mu_{\rm T}-\epsilon_{\rm T\mathbf{k}})$ and $n_{\rm S\mathbf{k}\sigma}=\langle c^\dagger_{\mathbf{k}\sigma}c_{\mathbf{k}\sigma}\rangle_{T=0}=\Theta(\mu_{\rm S}-\epsilon_{\rm S\mathbf{k}})$ with their respective chemical potentials $\mu_{\rm T}$ and $\mu_{\rm S}$. By applying a voltage between tip and substrate the chemical potentials change such that $\mu_{\rm T}=\mu_{\rm S}+eV$.

The elastic and inelastic tunneling currents calculated using (1.13), (1.14) are

$$\langle I_{1,\rm ext}(V)\rangle=\frac{4\pi Ae}{\hbar}\sum_{r_{\rm I}r'_{\rm I}r_{\rm S}r'_{\rm S}}t_1^*(r_{\rm I}-r_{\rm T})t_2(r_{\rm I}-r_{\rm S})t_1(r'_{\rm I}-r_{\rm T})t_2^*(r'_{\rm I}-r'_{\rm S})J_0(k_{\rm F}|r'_{\rm S}-r_{\rm S}|)\int d\epsilon\,(n_T(\epsilon)-n_S(\epsilon))\rho_T(\epsilon)\rho_S(\epsilon) \quad (1.15)$$

$$\langle I_{2,\rm ext}(V)\rangle=\frac{4\pi Be}{\hbar}\sum_{r_{\rm I}r'_{\rm I}r_{\rm S}r'_{\rm S}}t_1^*(r_{\rm I}-r_{\rm T})t_2(r_{\rm I}-r_{\rm S})t_1(r'_{\rm I}-r_{\rm T})t_2^*(r'_{\rm I}-r'_{\rm S})J_0(k_{\rm F}|r'_{\rm S}-r_{\rm S}|)\int d\epsilon_S\int d\epsilon_T\quad\rho_T(\epsilon_T)\rho_S(\epsilon_S)$$

$$\int_{-\infty}^{\infty}\frac{d\omega}{2\pi}\sum_\alpha\left(n_T(\epsilon_T)(1-n_S(\epsilon_S))\tilde{S}^{\alpha\alpha}_{r_{\rm I}r'_{\rm I}}(\omega)\delta(\epsilon_T-\epsilon_S-\hbar\omega)-n_S(\epsilon_S)(1-n_T(\epsilon_T))\tilde{S}^{\alpha\alpha}_{r_{\rm I}r'_{\rm I}}(\omega)\delta(\epsilon_T-\epsilon_S+\hbar\omega)\right). \quad (1.16)$$

In the above calculation we have assumed that the Fermi surface is spherical with radius a $k_{\rm F}$ and that tunneling can occur for momenta near this surface. With this assumption we can approximate as follows

$$\sum_{k}e^{i\mathbf{k}\cdot(r_{\rm S}-r'_{\rm S})}n_k f(\epsilon_k)=\int\frac{d^2\boldsymbol{k}}{(2\pi)^2}e^{i\mathbf{k}\cdot(r_{\rm S}-r'_{\rm S})}n_k f(\epsilon_k)$$

$$\simeq\int_0^{2\pi}d\phi\int_{-\Lambda}^{\Lambda}\frac{d(\delta k)}{2\pi}k_{\rm F}\exp\left(k_{\rm F}\hat{\boldsymbol{k}}\cdot(\boldsymbol{r}_{\rm S}-\boldsymbol{r}'_{\rm S})\right)n_k f(\epsilon_k)\simeq\frac{1}{2\pi}\int_0^{2\pi}d\phi\exp\left(k_{\rm F}\hat{\boldsymbol{k}}\cdot(\boldsymbol{r}_{\rm S}-\boldsymbol{r}'_{\rm S})\right)\int d\epsilon n(\epsilon)\rho(\epsilon)f(\epsilon) \quad (1.17)$$

and the above expression can be simplified using the integral representation of the Bessel function of first kind $J_0$

$$\frac{1}{2\pi}\int_0^{2\pi}d\phi\exp\left(k_{\rm F}\hat{\boldsymbol{k}}\cdot(\boldsymbol{r}_{\rm S}-\boldsymbol{r}'_{\rm S})\right)=J_0\left(k_{\rm F}|\boldsymbol{r}_{\rm S}-\boldsymbol{r}'_{\rm S}|\right). \quad (1.18)$$

Here $\rho_{\rm T}$ and $\rho_{\rm S}$ are the density of states at the tip and substrate respectively. As the energy scales in the magnetic system that we are dealing with are much smaller compared to the electronic energy scale (energy scale on which $\rho_{\rm T}$ and $\rho_{\rm S}$ change) we may assume that $\rho_{\rm T}=\rho_{\rm S}=\rho$ and is a constant.

The elastic and inelastic tunneling conductance into an extended substrate are

$$\langle G_{1,\mathrm{ext}}(V)\rangle = \frac{4\pi A e^2\rho^2}{\hbar}\sum_{\boldsymbol{r}_\mathrm{I}\boldsymbol{r}'_\mathrm{I}\boldsymbol{r}_\mathrm{S}\boldsymbol{r}'_\mathrm{S}}\sum_{ab} t_1^*(\boldsymbol{r}_\mathrm{Ia}-\boldsymbol{r}_\mathrm{T})t_2(\boldsymbol{r}_\mathrm{Ia}-\boldsymbol{r}_\mathrm{S})t_1(\boldsymbol{r}'_\mathrm{Ib}-\boldsymbol{r}_\mathrm{T})t_2^*(\boldsymbol{r}'_\mathrm{Ib}-\boldsymbol{r}'_\mathrm{S})J_0(k_\mathrm{F}|r'_\mathrm{S}-r_\mathrm{S}|) \tag{1.19}$$

$$\langle G_{2,\mathrm{ext}}(V)\rangle = \frac{4\pi B e^2\rho^2}{\hbar}\sum_{\boldsymbol{r}_\mathrm{I}\boldsymbol{r}'_\mathrm{I}\boldsymbol{r}_\mathrm{S}\boldsymbol{r}'_\mathrm{S}}\sum_{ab} t_1^*(\boldsymbol{r}_\mathrm{Ia}-\boldsymbol{r}_\mathrm{T})t_2(\boldsymbol{r}_\mathrm{Ia}-\boldsymbol{r}_\mathrm{S})t_1(\boldsymbol{r}'_\mathrm{Ib}-\boldsymbol{r}_\mathrm{T})t_2^*(\boldsymbol{r}'_\mathrm{Ib}-\boldsymbol{r}'_\mathrm{S})J_0(k_\mathrm{F}|r'_\mathrm{S}-r_\mathrm{S}|)\int_0^{eV} d\omega\sum_\alpha \tilde{S}^{\alpha\alpha}_{\boldsymbol{r}_\mathrm{Ia}\boldsymbol{r}'_\mathrm{Ib}}(\omega) \tag{1.20}$$

where

$$\sum_\alpha \tilde{S}^{\alpha\alpha}_{\boldsymbol{r}_\mathrm{Ia}\boldsymbol{r}'_\mathrm{Ib}}(\omega) = \frac{1}{2\pi}\int d\mathbf{k}\sum_\alpha S^{\alpha\alpha}_{ab}(\mathbf{k},\omega)e^{-i\mathbf{k}\cdot(\boldsymbol{r}_\mathrm{Ia}-\boldsymbol{r}'_\mathrm{Ib})}. \tag{1.21}$$

We now assume that the tunneling amplitudes $t_1$ and $t_2$ involve three length scales: $d$ which is a characteristic length scale for tunneling along $z$ direction and $\lambda_1$, $\lambda_2$ which are characteristic length scales for tunneling along the lateral directions such that

$$t_1(\boldsymbol{r}_\mathrm{I}-\boldsymbol{r}_\mathrm{T}) = \Gamma\exp(-d_1/d)\exp(-|\boldsymbol{r}_\mathrm{I}-\boldsymbol{r}_\mathrm{T}|/2\lambda_1) \tag{1.22}$$

$$t_2(\boldsymbol{r}_\mathrm{I}-\boldsymbol{r}_\mathrm{S}) = \Gamma\exp(-d_2/d)\exp(-|\boldsymbol{r}_\mathrm{I}-\boldsymbol{r}_\mathrm{S}|/2\lambda_2). \tag{1.23}$$

Now we consider the approximation where the extended nature of the substrate is neglected, so $\boldsymbol{r}_\mathrm{S} = \boldsymbol{r}_\mathrm{T}$ and that tunneling can occur to the substrate only at positions directly below the tip. This qualitatively gives the same voltage response (Fig. S1). To simplify the calculations we let $T(\boldsymbol{r}_\mathrm{I}-\boldsymbol{r}_\mathrm{T}) = t_1^*(\boldsymbol{r}_\mathrm{I}-\boldsymbol{r}_\mathrm{T})t_2(\boldsymbol{r}_\mathrm{I}-\boldsymbol{r}_\mathrm{T})$, and $\lambda = \lambda_1 = \lambda_2$. With these assumptions, using 1.15, 1.16 the elastic and inelastic tunneling current are

$$\langle I_1(V)\rangle = \frac{4\pi A e}{\hbar}\sum_{\boldsymbol{r}_\mathrm{I}\boldsymbol{r}'_\mathrm{I}} T(\boldsymbol{r}_\mathrm{I}-\boldsymbol{r}_\mathrm{T})T(\boldsymbol{r}'_\mathrm{I}-\boldsymbol{r}_\mathrm{T})\int d\epsilon\,(n_T(\epsilon)-n_S(\epsilon))\rho_T(\epsilon)\rho_S(\epsilon) \tag{1.24}$$

$$\langle I_2(V)\rangle = \frac{4\pi B e}{\hbar}\sum_{\boldsymbol{r}_\mathrm{I}\boldsymbol{r}'_\mathrm{I}}\int d\epsilon_S\int d\epsilon_T\quad \rho_T(\epsilon_T)\rho_S(\epsilon_S)T(\boldsymbol{r}_\mathrm{I}-\boldsymbol{r}_\mathrm{T})T(\boldsymbol{r}'_\mathrm{I}-\boldsymbol{r}_\mathrm{T})$$

$$\int_{-\infty}^{\infty}\frac{d\omega}{2\pi}\sum_i\Big(n_T(\epsilon_T)(1-n_S(\epsilon_S))\tilde{S}^{ii}_{\boldsymbol{r}_\mathrm{I}\boldsymbol{r}'_\mathrm{I}}(\omega)\delta(\epsilon_T-\epsilon_S-\hbar\omega) - n_S(\epsilon_S)(1-n_T(\epsilon_T))\tilde{S}^{ii}_{\boldsymbol{r}_\mathrm{I}\boldsymbol{r}'_\mathrm{I}}(\omega)\delta(\epsilon_T-\epsilon_S+\hbar\omega)\Big) \tag{1.25}$$

Again we assume $\rho_\mathrm{T} = \rho_\mathrm{S} = \rho$, a constant, and $T(\boldsymbol{r}_\mathrm{I}-\boldsymbol{r}_\mathrm{T}) = \Gamma^2\exp\left(-(d_1+d_2)/d\right)\exp\left(-|\boldsymbol{r}_\mathrm{I}-\boldsymbol{r}_\mathrm{T}|/\lambda\right)$. So we calculate the elastic and inelastic contribution to the tunneling conductance as

$$\langle G_1(V)\rangle = \frac{4\pi A e^2\rho^2\Gamma^4}{\hbar}\exp(-2(d_1+d_2)/d)\sum_{ab}\sum_{\boldsymbol{r}_\mathrm{I}\boldsymbol{r}'_\mathrm{I}} e^{-\frac{2}{\lambda}(|\boldsymbol{r}_\mathrm{Ia}-\boldsymbol{r}_\mathrm{T}|+|\boldsymbol{r}'_\mathrm{Ib}-\boldsymbol{r}_\mathrm{T}|)} \tag{1.26}$$

$$\langle G_2(V)\rangle = \frac{4\pi B e^2\rho^2\Gamma^4}{\hbar}\exp(-2(d_1+d_2)/d)\sum_{ab}\sum_{\boldsymbol{r}_\mathrm{I}\boldsymbol{r}'_\mathrm{I}} e^{-\frac{2}{\lambda}(|\boldsymbol{r}_\mathrm{Ia}-\boldsymbol{r}_\mathrm{T}|+|\boldsymbol{r}'_\mathrm{Ib}-\boldsymbol{r}_\mathrm{T}|)}\int_0^{eV} d\omega\sum_\alpha \tilde{S}^{\alpha\alpha}_{\boldsymbol{r}_\mathrm{Ia}\boldsymbol{r}'_\mathrm{Ib}}(\omega). \tag{1.27}$$

In subsequent sections and figures we take $G_0 \equiv \frac{4\pi B e^2\rho^2\Gamma^4}{\hbar}\exp(-2(d_1+d_2)/d)$ and, for simplicity, $a/\lambda = 1$.

## 2. INELASTIC TUNNELING

### 2.1. Spin Wave Theory

We now turn to the calculation of the dynamical spin-spin correlator that is the principal ingredient in the calculation of the tunneling conductance. To do this, we suppose that the local moments in the magnetic layer are polarized - either spontaneously or in the presence of a magnetic field. We then carry out a spin wave expansion around the ordered magnetic texture using the Holstein-Primakoff representation of spins of length $S$ [8]

$$\hat{S}^z = S - \hat{a}^\dagger\hat{a} \tag{2.1}$$

$$\hat{S}^+ = \sqrt{2S}\sqrt{1-\frac{\hat{a}^\dagger\hat{a}}{2S}}\hat{a} = \sqrt{2S}\left(1-\frac{\hat{a}^\dagger\hat{a}}{4S}\right)\hat{a}+\ldots \tag{2.2}$$

$$\hat{S}^- = \sqrt{2S}\hat{a}^\dagger\sqrt{1-\frac{\hat{a}^\dagger\hat{a}}{2S}} = \sqrt{2S}\hat{a}^\dagger\left(1-\frac{\hat{a}^\dagger\hat{a}}{4S}\right)+\ldots \tag{2.3}$$

where the bosons satisfy the usual commutation relations $[\hat{a}, \hat{a}^\dagger] = 1$.

Expanding about the mean field ground state with $\hat{\mathbf{z}}_m$ as the local quantization on magnetic sublattice $m$ we obtain the quadratic Hamiltonian

$$\mathsf{H}_{\mathsf{SW}} = \frac{S}{2}\sum_{\boldsymbol{k}} \hat{\boldsymbol{\Psi}}^\dagger(\boldsymbol{k}) \begin{pmatrix} \mathsf{A}(\boldsymbol{k}) & \mathsf{B}(\boldsymbol{k}) \\ \mathsf{B}^\star(-\boldsymbol{k}) & \mathsf{A}^\star(-\boldsymbol{k}) \end{pmatrix} \hat{\boldsymbol{\Psi}}(\boldsymbol{k}) \equiv \frac{S}{2}\sum_{\boldsymbol{k}} \hat{\boldsymbol{\Psi}}^\dagger(\boldsymbol{k}) \boldsymbol{M}(\boldsymbol{k}) \hat{\boldsymbol{\Psi}}(\boldsymbol{k}) \tag{2.4}$$

where

$$\hat{\boldsymbol{\Psi}}^\dagger(\boldsymbol{k}) = \begin{pmatrix} \hat{a}^\dagger_{\boldsymbol{k}1} \ldots \hat{a}^\dagger_{\boldsymbol{k}m}\, \hat{a}_{-\boldsymbol{k}1} \ldots \hat{a}_{-\boldsymbol{k}m} \end{pmatrix} \quad \hat{\boldsymbol{\Psi}}(\boldsymbol{k}) = \begin{pmatrix} \hat{a}_{\boldsymbol{k}1} \\ \vdots \\ \hat{a}_{\boldsymbol{k}m} \\ \hat{a}^\dagger_{-\boldsymbol{k}1} \\ \vdots \\ \hat{a}^\dagger_{-\boldsymbol{k}m} \end{pmatrix} \tag{2.5}$$

and the number conserving terms $\mathsf{A}_{ab}(\boldsymbol{k})$ and number non-conserving terms $\mathsf{B}_{ab}(\boldsymbol{k})$ depend on the exchange couplings in the local frame.

To obtain the spectrum and magnon wavefunctions we diagonalize the Hamiltonian (2.4) using a free boson Bogoliubov transformation: $T^{-1}(\boldsymbol{k})M(\boldsymbol{k})T(\boldsymbol{k}) = \Lambda(\boldsymbol{k})$ where $\Lambda(\mathbf{k})$ is diagonal and the entries of the $M(\boldsymbol{k})$ depend on the model under consideration. The dynamical structure factor is calculated directly from linear spin wave theory. The sublattice resolved structure factor is defined as

$$S_{ab}(\mathbf{k}, \omega) = \frac{1}{n_s}\sum_{\alpha} S^{\alpha\alpha}_{ab}(\mathbf{k}, \omega) \tag{2.6}$$

$$S^{\alpha\beta}_{ab}(\mathbf{k}, \omega) = \frac{1}{N}\sum_{n}\sum_{i,j} \langle 0| S^{\alpha}_{ia} |n\rangle \langle n| S^{\beta}_{jb} |0\rangle \exp[i\mathbf{k}\cdot(\mathbf{R}_{\mathrm{ia}} - \mathbf{R}_{\mathrm{jb}})]\delta(\omega - \epsilon^{(n)}_{\mathbf{k}}) \tag{2.7}$$

where $a, b$ are sublattice indices and $\mathbf{R}_{\mathrm{ia}} = \mathbf{R}_{\mathrm{i}} + \mathbf{r}_{\mathrm{a}}$ where $\mathbf{R}_{\mathrm{i}}$ is the position of the primitive site $i$ and $\mathbf{r}_{\mathrm{a}}$ is the basis vector for that sublattice. The modes are $\epsilon^{(n)}_{\mathbf{k}}$ for $n = 1, \ldots, n_s$, where $n_s$ is the number of sub-lattices. Calculated to linear order in spin wave theory, the transverse components give a single-magnon contribution, while $S^{zz}$ gives a two-magnon continuum contribution to the dynamical structure factor.

### 2.2. Models

We consider three qualitatively distinct scenarios for the magnetic excitations to explore the range of possible phenomena potentially observable using tunneling spectroscopy. These include the square lattice antiferromagnet that has a linear dispersing Goldstone mode and a single band, the honeycomb lattice ferromagnet that has two bands joined by Dirac points and the Heisenberg-Kitaev model in the polarized phase where the two bands are gapped and topological and the ground state is unstable to the introduction of impurities.

#### *2.2.1. Square Lattice Heisenberg Antiferromagnet*

This classic nearest neighbor model with Hamiltonian

$$H_{AFM} = J\sum_{<i,j>} \mathbf{S_i}\cdot\mathbf{S_j} \tag{2.8}$$

and $J > 0$ has a Neel ordered ground state. Expanding around the mean field ground state, the corresponding $M(k)$ matrix has

$$A(\boldsymbol{k}) = \begin{pmatrix} 4JS & 0 \\ 0 & 4JS \end{pmatrix} \tag{2.9}$$

$$B(\boldsymbol{k}) = \begin{pmatrix} 0 & 4JS\gamma(\boldsymbol{k}) \\ 4JS\gamma(\boldsymbol{k}) & 0 \end{pmatrix} \tag{2.10}$$

where $\gamma(\mathbf{k}) = \frac{1}{2}(\cos k_x + \cos k_y) \equiv \tanh 2\theta_{\mathbf{k}}$. One finds a single magnon band with dispersion $\epsilon_{\mathbf{k}} = 4JS\sqrt{1-\gamma(\mathbf{k})^2}$ and a band-width $4JS$. The two-magnon continuum has twice this band width. The dispersion relation is linearised near the $\Gamma$ point as $\epsilon_{\mathbf{k}} = 2\sqrt{2}JS|\mathbf{k}|$.

For this model, the dynamical structure factor is

$$S(\mathbf{k},\omega) = S(\cosh 2\theta_{\mathbf{k}} - \sinh 2\theta_{\mathbf{k}})\delta(\omega-\epsilon_{\mathbf{k}}) + \frac{1}{2}\sum_{\mathbf{q}}(\cosh\theta_{\mathbf{q}}\sinh\theta_{\mathbf{k}-\mathbf{q}} - \cosh\theta_{\mathbf{k}-\mathbf{q}}\sinh\theta_{\mathbf{q}})^2\delta(\omega-\epsilon_{\mathbf{q}}-\epsilon_{\mathbf{k}-\mathbf{q}}). \tag{2.11}$$

The dynamical structure factor on the single-magnon band has a divergent intensity $\propto \frac{1}{|\mathbf{k}-\mathbf{k}_R|}$ near the $R$ of the first Brillouin zone, while near the $\Gamma$ it is linearised as $S(\mathbf{k},\omega) \approx \frac{S}{2\sqrt{2}}|\mathbf{k}|\delta(\omega - 2\sqrt{2}JS|\mathbf{k}|)$.

### *2.2.2. Kitaev-Heisenberg Honeycomb*

The second model we consider is the Kitaev-Heisenberg model on a honeycomb lattice with nearest neighbor interactions in the presence of a magnetic field $\mathbf{h}$. We consider the magnetic field to be perpendicular to the plane of the honeycomb layer (i.e. in the [111] direction).

$$H_{KH} = J\sum_{<i,j>}\mathbf{S}_i\cdot\mathbf{S}_j + \sum_{<i,j>^\gamma}2KS_i^\gamma S_j^\gamma - \mathbf{h}\cdot\sum_i\mathbf{S}_i \tag{2.12}$$

where $\gamma$ has label $x, y, z$ depending on the orientation of the bond. We parametrize the Hamiltonian with $J = \cos\theta$ and $K = \sin\theta$. We work in the polarized phase above some threshold field that depends on the coupling $\theta$. The corresponding $M(\boldsymbol{k})$ matrix has

$$A(\mathbf{k}) = \begin{pmatrix} -3JS - 2KS + h & \left(J+\frac{2K}{3}\right)S\left(e^{+i\mathbf{k}\cdot\delta_x} + e^{+i\mathbf{k}\cdot\delta_y} + e^{+i\mathbf{k}\cdot\delta_z}\right) \\ \left(J+\frac{2K}{3}\right)S\left(e^{-i\mathbf{k}\cdot\delta_x} + e^{-i\mathbf{k}\cdot\delta_y} + e^{-i\mathbf{k}\cdot\delta_z}\right) & -3JS - 2KS + h \end{pmatrix} \tag{2.13}$$

$$B(\mathbf{k}) = \begin{pmatrix} 0 & \frac{2KS}{3}\left(e^{+i\mathbf{k}\cdot\delta_x - \frac{2\pi i}{3}} + e^{+i\mathbf{k}\cdot\delta_y + \frac{2\pi i}{3}} + e^{+i\mathbf{k}\cdot\delta_z}\right) \\ \frac{2KS}{3}\left(e^{-i\mathbf{k}\cdot\delta_x - \frac{2\pi i}{3}} + e^{-i\mathbf{k}\cdot\delta_y + \frac{2\pi i}{3}} + e^{-i\mathbf{k}\cdot\delta_z}\right) & 0 \end{pmatrix} \tag{2.14}$$

where $\delta_x = (-1, 0)$, $\delta_y = (1/2, -\sqrt{3}/2)$ and $\delta_z = (1/2, \sqrt{3}/2)$.

At the special values of $\theta$ for which the Kitaev coupling vanishes, $\theta = \pi$ and $\theta = 0$, the spectrum has Dirac points at the $K$ points. When the Kitaev coupling is switched on a band gap opens between the two magnon bands and each band carries a nonzero Chern number with the consequence that the introduction of a boundary leads to the presence of chiral magnon modes within the band gap and localized at the surface [9, 10].

For the special case of the Heisenberg ferromagnet ($\theta = \pi$) the dispersion relations are $\epsilon^{(1)}_{\mathbf{k}} = JS(3 - |\gamma(\mathbf{k})|)$ and $\epsilon^{(2)}_{\mathbf{k}} = JS(3 + |\gamma(\mathbf{k})|)$ for the lower and upper modes respectively, where $\gamma(\mathbf{k}) = e^{-i\mathbf{k}\cdot\delta_x} + e^{-i\mathbf{k}\cdot\delta_y} + e^{-i\mathbf{k}\cdot\delta_z}$ with $\delta_x = (-1, 0)$, $\delta_y = \left(\frac{1}{2}, \frac{\sqrt{3}}{2}\right)$, $\delta_z = \left(\frac{1}{2}, \frac{-\sqrt{3}}{2}\right)$ being vectors along along the three types of bonds in the honeycomb lattice. Near the $\Gamma$ point $\epsilon^{(1)}_{\mathbf{k}} \approx \frac{3JS}{4}|\mathbf{k}|^2$ and $\epsilon^{(2)}_{\mathbf{k}} \approx JS\left(6 - \frac{3}{4}|\mathbf{k}|^2\right)$ for small $\mathbf{k}$. The two-bands only touch at the $K$ point (Dirac point) of the first BZ. The analytic form of the dynamical structure factor is

$$S(\mathbf{k},\omega) = S\left(1 - \frac{\mathrm{Re}[\gamma(\mathbf{k})]}{|\gamma(\mathbf{k})|}\right)\delta(\omega - \epsilon^{(1)}_{\mathbf{k}}) + S\left(1 + \frac{\mathrm{Re}[\gamma(\mathbf{k})]}{|\gamma(\mathbf{k})|}\right)\delta(\omega - \epsilon^{(2)}_{\mathbf{k}}). \tag{2.15}$$

## 3. TUNNELING IN THE CLEAN SYSTEM

### 3.1. Method

The tip is placed directly above one of lattice points in the impurity layer and we probe the inelastic tunneling conductance $G_2(V)$ as a function of voltage. The elastic tunneling conductance $G_1(V)$ gives a constant background due to its Ohmic nature, and so we do not take it into account. As we probe the system in the bulk, we consider it to be translationally invariant and so the tunneling conductance if probed at any of the lattice sites will be the same.

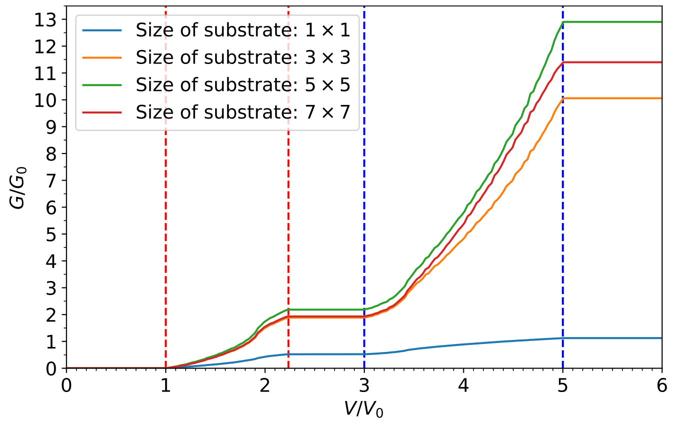


FIG. S1. Normalized tunneling conductance $G/G_0$ including the contribution from an extended substrate plotted as a function of bias voltage $V$ ($V_0 = JS/e$) for the Kitaev-Heisenberg model $\theta = \pi/2$, $h = 5$ on a honeycomb lattice (with $k_F = 1/a$). The metallic substrate is a square lattice and tunneling is possible to all sites below the STM tip. The saturation value of $G/G_0$ converges with increasing size of substrate, the oscillatory behaviour is due to the presence of Bessel function $J_0$ in (1.20).

First we consider that tunneling is allowed into the substrate to a small patch directly below the STM tip (Fig. S1). Increasing the size of this patch increases the conductance (S1) as the number of accessible sites increases and more channels become available for tunneling. However the important qualitative features are still visible by allowing the smallest possible patch ($1 \times 1$) on the substrate.

Henceforth we work in the approximation that tunneling can occur into the substrate only at $\boldsymbol{r}_{\mathrm{T}}$ that is the point directly below the STM tip.

### 3.2. Results

*Heisenberg antiferromagnet*: The one-magnon contribution to inelastic tunneling conductance for this model increases monotonously with applied voltage from zero to its maximum value (Fig. S2), as the voltage is varied across the extent of the bandwidth, $V = 4JS$. This variation is qualitatively similar to that of the cumulative density of states with voltage. However, if the continuum contribution is also taken into account the inelastic part of the tunneling conductance saturates at $V = 8JS$ (Fig. S3), which is the extent of the continuum. The continuum contribution to the tunneling conductance is an order of magnitude smaller than the one-magnon contribution.

*Kitaev-Heisenberg on honeycomb lattice*: $\theta = \frac{\pi}{2}$: Here there are two magnon bands and the extent of each can be clearly distinguished through STM (Fig. S2). The inelastic tunneling conductance plateaus in the gap between these two bands, which is equivalent to the gap between their spectra at the $K$ point of the hexagonal BZ.

$\theta = 0, \pi$: There are again two magnon bands which touch at the $K$ point of the zone to form a Dirac point (bands are linearly dispersing around $K$). This shows up as an inflection point (Fig. S2) in both the inelastic tunneling conductance and the cumulative density of states. So again the extents of both the bands can be determined.

The two-magnon continuum contribution is present only when the Hamiltonian has number non-conserving terms. So it only shows up when the Kitaev coupling is nonzero (Fig. S3). Taking the continuum contribution into account reveals that at low $\mathbf{h}$ it may obscure the exact variation of the one-magnon tunneling conductance, by making it difficult to identify the inter-band plateaus in the conductance. Although this problem may be alleviated by working at high $\mathbf{h}$ so that the lowest energy of the continuum is higher than the top of the upper magnon band.

In summary, by probing the inelastic tunneling conductance in a clean system we are able to find (i) the number of magnon bands in the sample, (ii) the bandwidths of each band, (iii) the magnitude of the inter-band gaps in the single-magnon spectrum. Also we verify that the variation of the inelastic tunneling conductance mimics the variation of the cumulative density of states with voltage.

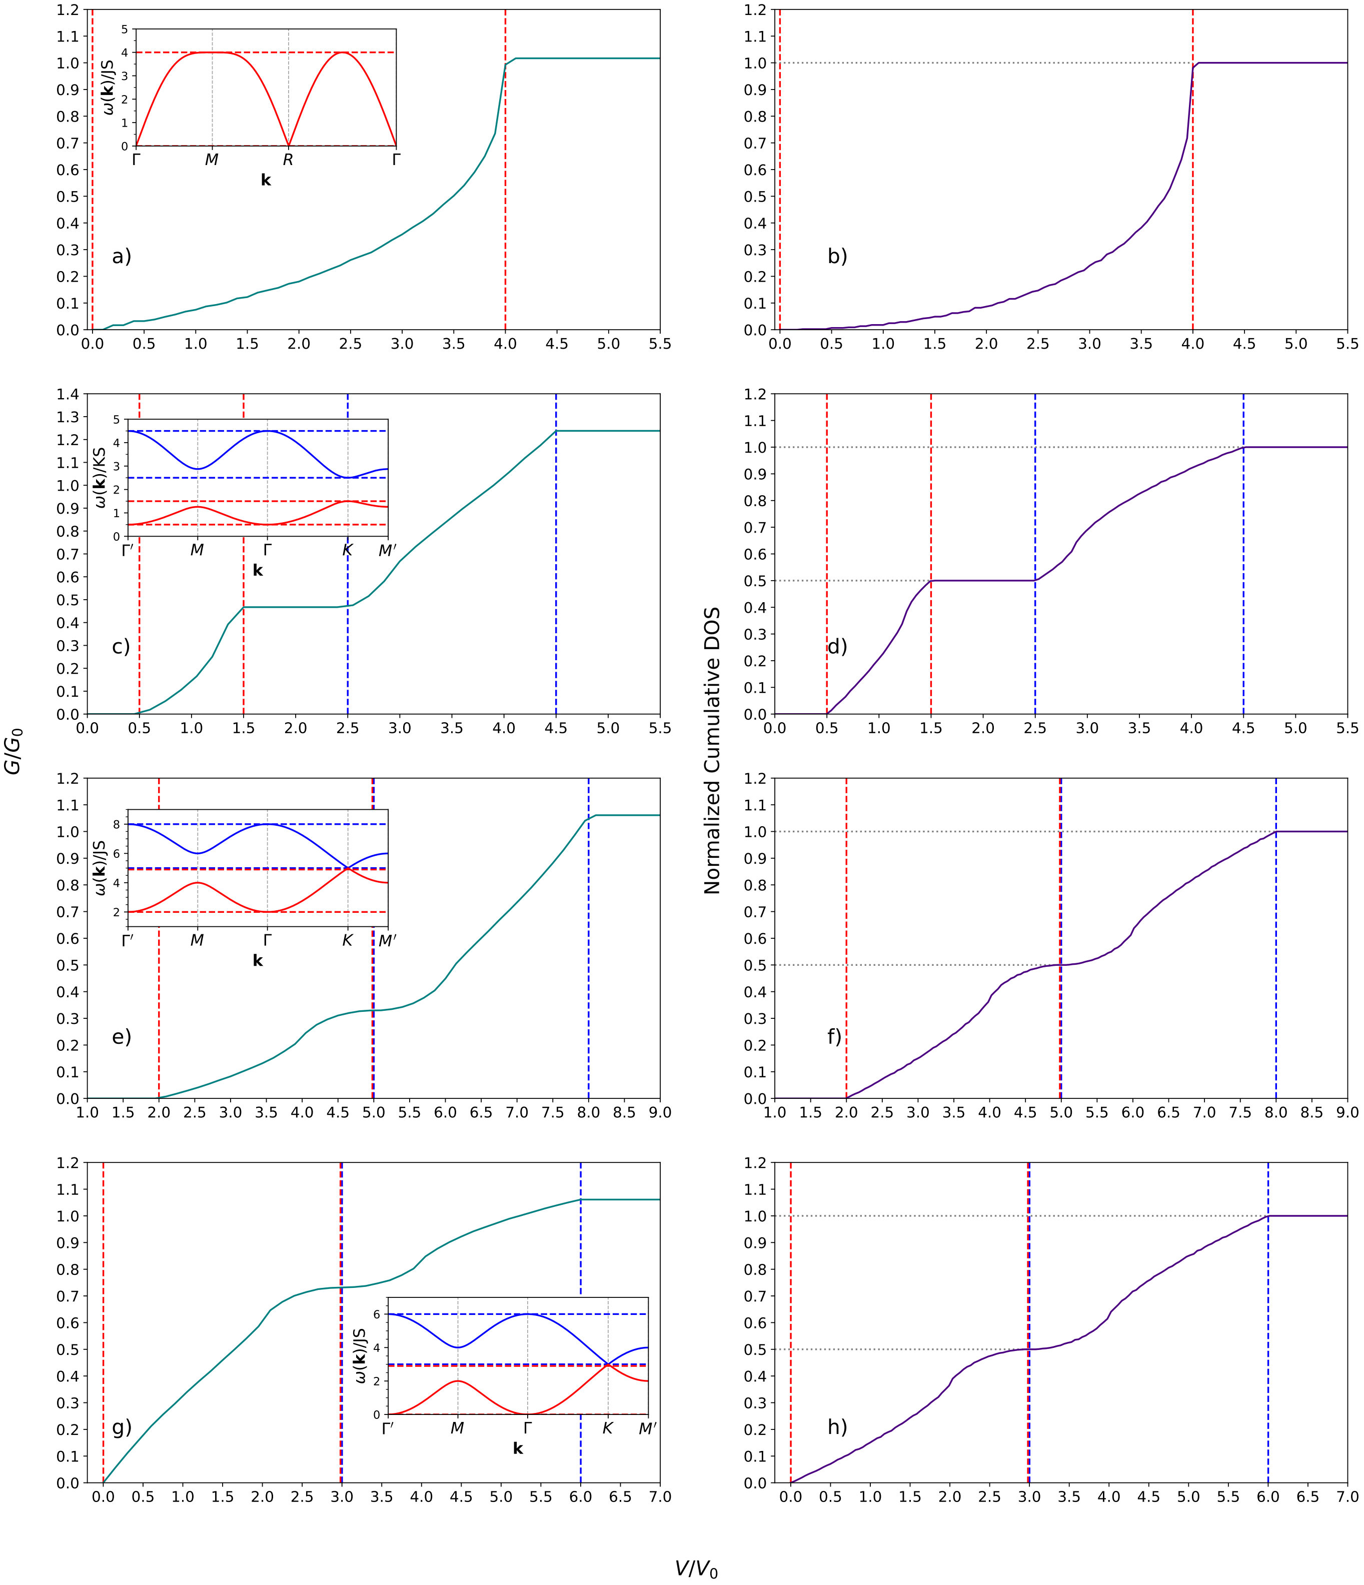


FIG. S2. Normalized inelastic tunneling conductance $G/G_0$ and cumulative density of states plotted as a function of bias voltage $V$ for different models including scattering from single-magnon states: (a) & (b) the square lattice antiferromagnet, (c) & (d) the Kitaev-Heisenberg model with $\theta = \pi/2$, h=4.5, (e) & (f) the Heisenberg honeycomb antiferromagnet in finite field at $\theta = 0$, $h = 7$ and, (g) & (h) the Heisenberg honeycomb ferromagnet in zero field at $\theta = \pi$, $h = 0$. The insets show the dispersion relations along the indicated high symmetry directions in reciprocal space. Dashed lines indicate the band edges.

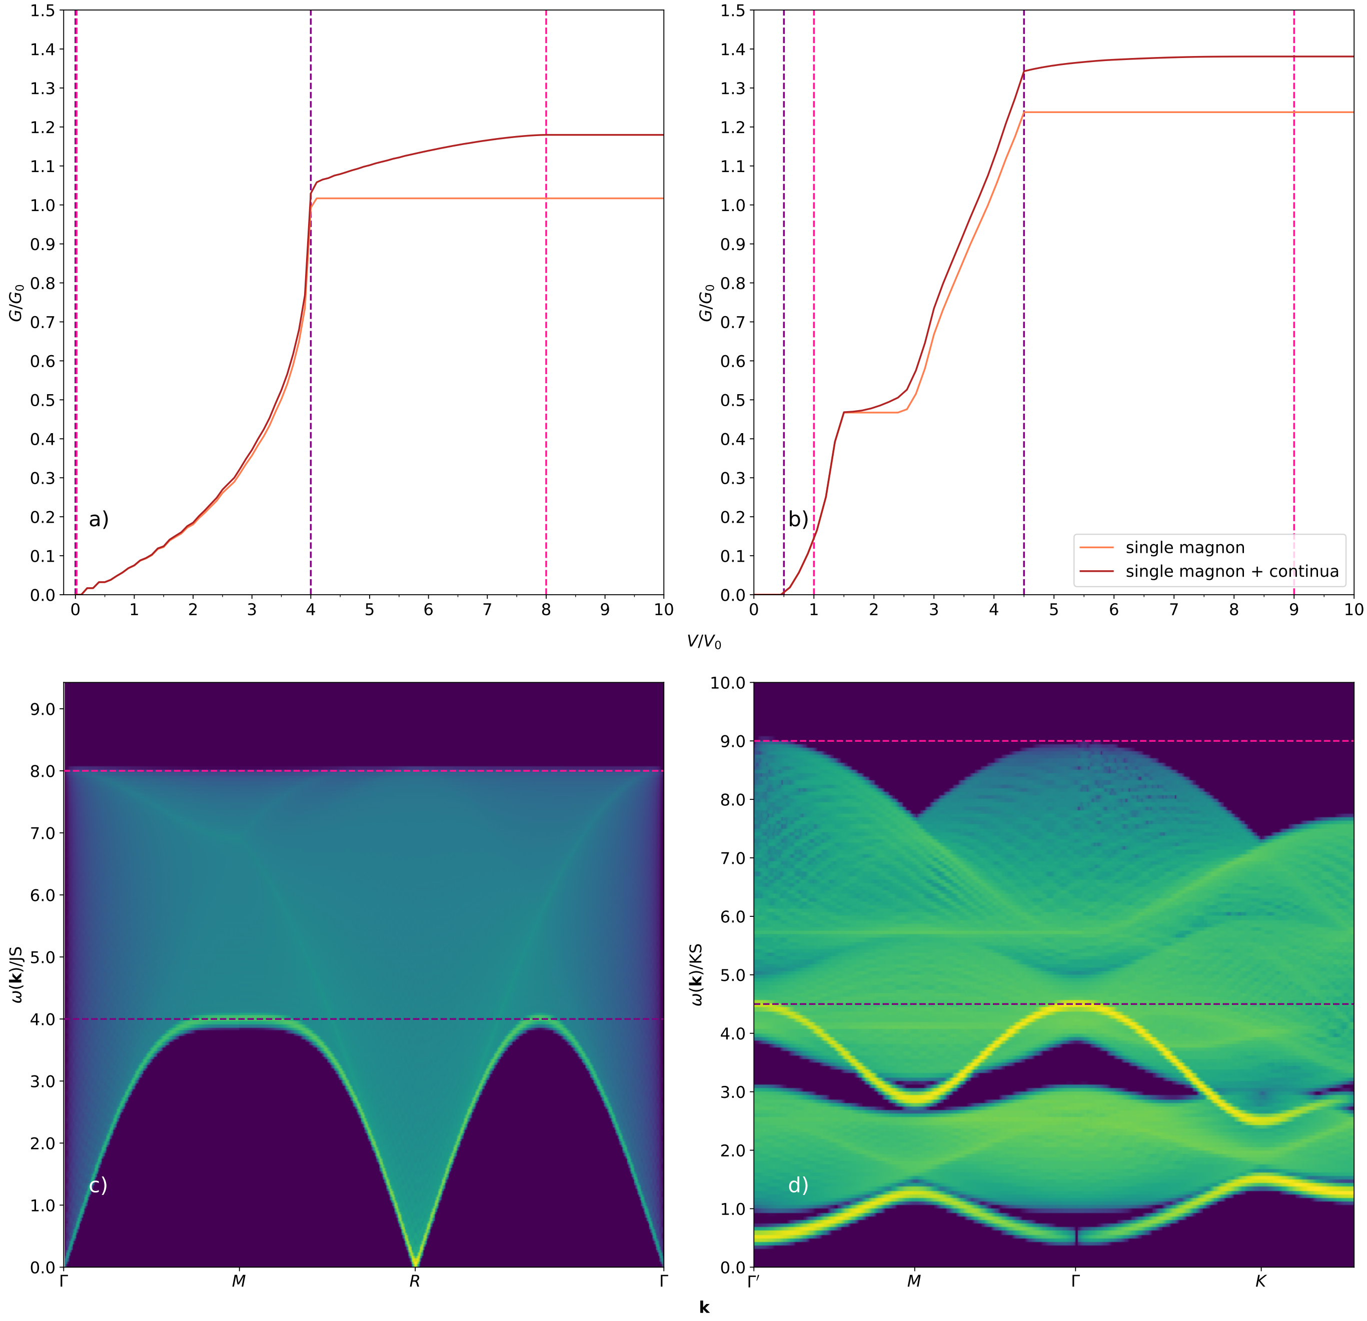


FIG. S3. Normalized tunneling conductance $G/G_0$ plotted as a function of bias voltage $V$ for different models to illustrate the effect of including the two-magnon contribution to the tunneling. (a) Plot for the square lattice antiferromagnet showing that the principal two-magnon contribution appears for energies above the upper single-magnon band edge although the continuum extends from zero energy up to $8JS$. (b) Plot for the Heisenberg-Kitaev model for $\theta = \pi/2$ showing a significant continuum contribution within the single-magnon band gap. Dashed lines indicate the boundaries of the single- and two- magnon states. Plots of the dynamical structure factor for single- and two-magnons: (c) Square lattice antiferromagnet, (d) Kitaev-Heisenberg with $\theta = \pi/2$ and $h = 4.5$

## 4. IMPURITY SCATTERING

### 4.1. Methods

We compute the tunneling conductance in two different ways. The first method is to numerically diagonalize the linear spin wave Hamiltonian on a slab (21×21) with periodic boundary conditions and, from the resulting spectrum, compute the dynamical

spin-spin correlator.

A second method – that is applicable to the case where the ground state is stable to the presence of an impurity – is to use the exact infinite un-disordered system single-particle Green's functions to compute their analogs exactly in the presence of an impurity [11].

Starting from the Hamiltonian in real space

$$\hat{H} = \frac{1}{2}\sum_{i,j}\left(a_1^\dagger \ldots a_N^\dagger a_1 \ldots a_N\right) H_{ij,ab}\begin{pmatrix} a_1 \\ .. \\ a_N \\ a_1^\dagger \\ .. \\ a_N^\dagger \end{pmatrix} \tag{4.1}$$

where $i, j$ label sites and $a, b$ label the blocks distinguishing between number conserving and non-conserving terms and the boson operators are Holstein-Primakoff bosons. Then, defining the matrix of single particle Green's functions

$$\mathcal{G}_{ij}(\tau) \equiv \begin{pmatrix} -\left\langle \mathcal{T}\left[a_i^\dagger(\tau)a_j(0)\right]\right\rangle & -\left\langle \mathcal{T}\left[a_i^\dagger(\tau)a_j^\dagger(0)\right]\right\rangle \\ -\left\langle \mathcal{T}\left[a_i(\tau)a_j(0)\right]\right\rangle & -\left\langle \mathcal{T}\left[a_i(\tau)a_j^\dagger(0)\right]\right\rangle \end{pmatrix} \tag{4.2}$$

one may show that

$$(\boldsymbol{\sigma}_3\partial_\tau - H)\,\mathcal{G} = \delta(\tau) \tag{4.3}$$

where $\boldsymbol{\sigma}_3$ acts on the $a, b$ blocks.

Now we consider an impurity problem $\hat{H} = \hat{H}_0 + \hat{V}$ where $\hat{H}_0$ is the (non-interacting) Hamiltonian of the clean system and $\hat{V}$ is the (quadratic) impurity potential. Writing

$$(\boldsymbol{\sigma}_3\partial_\tau - H_0)\,\mathcal{G}_0 = \delta(\tau) \tag{4.4}$$

for the Green's functions in the clean system and identifying the left-hand sides of Eqs. 4.3 and 4.4 we obtain an integral equation for $\mathcal{G}$. Going to the (Matsubara) frequency domain via

$$\mathcal{G}(i\omega_n) = \int_0^\beta d\tau \mathcal{G}(\tau) e^{i\omega_n\tau} \tag{4.5}$$

we obtain the main result

$$[\mathcal{G}(i\omega_n)]_{ij} = [\mathcal{G}_0(i\omega_n)]_{ij} + [\mathcal{G}(i\omega_n)]_{im}\, V_{mn}\, [\mathcal{G}_0(i\omega_n)]_{nj}\,. \tag{4.6}$$

By repeatedly iterating the substitution of $\mathcal{G}(i\omega_n)$ on the right-hand-side one sees the physical interpretation of this expression as the infinite sum of elastic magnon scattering events from the impurity potential.

*Square Lattice Heisenberg Antiferromagnet* – The relevant (Matsubara single particle) Green's functions for the problem of the square lattice antiferromagnet are

$$G_{ij}(\tau) \equiv \begin{pmatrix} -\left\langle \mathcal{T}\left[a_i^\dagger(\tau)a_j(0)\right]\right\rangle & -\left\langle \mathcal{T}\left[a_i^\dagger(\tau)b_j^\dagger(0)\right]\right\rangle \\ -\left\langle \mathcal{T}\left[b_i(\tau)a_j(0)\right]\right\rangle & -\left\langle \mathcal{T}\left[b_i(\tau)b_j^\dagger(0)\right]\right\rangle \end{pmatrix} \tag{4.7}$$

where $a$ and $b$ are, respectively, Holstein-Primakoff bosons on the $A$ and $B$ sublattices. We write the Green's functions as $G_0$ when there are no impurities. One can show that

$$G_0^{11}(\boldsymbol{k}, \omega_n) = \frac{i\omega_n + 4JS}{(i\omega_n)^2 - \epsilon_{\boldsymbol{k}}^2} \tag{4.8}$$

and

$$G_0^{12}(\boldsymbol{k}, \omega_n) = -\frac{\gamma_{\boldsymbol{k}}}{(i\omega_n)^2 - \epsilon_{\boldsymbol{k}}^2}. \tag{4.9}$$

We take out a single spin at the origin on an A sublattice. This means that the impurity Hamiltonian is

$$V_{\mathrm{SLAFM}} = -J\sum_{\langle i,j\rangle} \boldsymbol{S}_0 \cdot (\boldsymbol{S}_1 + \boldsymbol{S}_2 + \boldsymbol{S}_3 + \boldsymbol{S}_4) \tag{4.10}$$

where the 0 site is at 0, 0 and the neighboring sites are labelled 1, 2, 3 and 4. After bosonizing we get

$$-4JS\,a_0^\dagger a_0 - JS\left(b_1^\dagger b_1 + b_2^\dagger b_2 + b_3^\dagger b_3 + b_4^\dagger b_4\right) - JS\left(a_0 b_1 + a_0 b_2 + a_0 b_3 + a_0 b_4 + \text{h.c.}\right). \tag{4.11}$$

It follows that the impurity Green's functions may be evaluated from the following equations by matrix inversion

$$[\mathcal{G}_{11}(i\omega_n)]_{jj'} = \left[\mathcal{G}^0_{11}(i\omega_n)\right]_{jj'} - JS\sum_\delta [\mathcal{G}_{12}(i\omega_n)]_{j\delta}\left(\left[\mathcal{G}^0_{21}(i\omega_n)\right]_{\delta j'} + \left[\mathcal{G}^0_{11}(i\omega_n)\right]_{0j'}\right) \tag{4.12}$$

$$[\mathcal{G}_{12}(i\omega_n)]_{jj'} = \left[\mathcal{G}^0_{12}(i\omega_n)\right]_{jj'} - JS\sum_\delta [\mathcal{G}_{12}(i\omega_n)]_{j\delta}\left(\left[\mathcal{G}^0_{22}(i\omega_n)\right]_{\delta j'} + \left[\mathcal{G}^0_{12}(i\omega_n)\right]_{0j'}\right) \tag{4.13}$$

$$[\mathcal{G}_{21}(i\omega_n)]_{jj'} = \left[\mathcal{G}^0_{21}(i\omega_n)\right]_{jj'} - JS\sum_\delta [\mathcal{G}_{22}(i\omega_n)]_{j\delta}\left(\left[\mathcal{G}^0_{21}(i\omega_n)\right]_{\delta j'} + \left[\mathcal{G}^0_{11}(i\omega_n)\right]_{0j'}\right) \tag{4.14}$$

$$[\mathcal{G}_{22}(i\omega_n)]_{jj'} = \left[\mathcal{G}^0_{22}(i\omega_n)\right]_{jj'} - JS\sum_\delta [\mathcal{G}_{22}(i\omega_n)]_{j\delta}\left(\left[\mathcal{G}^0_{22}(i\omega_n)\right]_{\delta j'} + \left[\mathcal{G}^0_{12}(i\omega_n)\right]_{0j'}\right) \tag{4.15}$$

after Eq. 4.6.

*Honeycomb Lattice Heisenberg Ferromagnet* – As before we define Green's functions

$$G_{ij}(\tau) \equiv \begin{pmatrix} -\left\langle \mathcal{T}\left[a_i(\tau)a_j^\dagger(0)\right]\right\rangle & -\left\langle \mathcal{T}\left[a_i(\tau)b_j^\dagger(0)\right]\right\rangle \\ -\left\langle \mathcal{T}\left[b_i(\tau)a_j^\dagger(0)\right]\right\rangle & -\left\langle \mathcal{T}\left[b_i(\tau)b_j^\dagger(0)\right]\right\rangle \end{pmatrix} \tag{4.16}$$

and one may show that

$$\mathcal{G}_{11}(\omega_n) = \mathcal{G}_{22}(\omega_n) = \frac{1}{2}\left(\frac{1}{i\omega_n - \epsilon^{(2)}_{\boldsymbol{k}}} + \frac{1}{i\omega_n - \epsilon^{(1)}_{\boldsymbol{k}}}\right) \tag{4.17}$$

and

$$\mathcal{G}_{12}(\omega_n) = \frac{e^{i\phi_k}}{2}\left(\frac{1}{i\omega_n - \epsilon^{(2)}_{\boldsymbol{k}}} + \frac{1}{i\omega_n - \epsilon^{(1)}_{\boldsymbol{k}}}\right) \tag{4.18}$$

and

$$\mathcal{G}_{21}(\omega_n) = \frac{e^{-i\phi_k}}{2}\left(\frac{1}{i\omega_n - \epsilon^{(2)}_{\boldsymbol{k}}} + \frac{1}{i\omega_n - \epsilon^{(1)}_{\boldsymbol{k}}}\right). \tag{4.19}$$

Now suppose we remove a single magnetic site 0 on the A sublattice. In real space we have $H_{\text{LSW+Imp}} = H_{\text{LSW}} + V$ with

$$V = -|J|S\left(3a_0^\dagger a_0 + b_1^\dagger b_1 + b_2^\dagger b_2 + b_3^\dagger b_3\right) + |J|S\left(a_0 b_1^\dagger + a_0 b_2^\dagger + a_0 b_3^\dagger + \text{h.c.}\right). \tag{4.20}$$

This leads to

$$[\mathcal{G}_{11}(i\omega_n)]_{jj'} = \left[\mathcal{G}^0_{11}(i\omega_n)\right]_{jj'} - |J|S\sum_\delta [\mathcal{G}_{12}(i\omega_n)]_{j\delta}\left(\left[\mathcal{G}^0_{21}(i\omega_n)\right]_{\delta j'} - \left[\mathcal{G}^0_{11}(i\omega_n)\right]_{0j'}\right) \tag{4.21}$$

$$[\mathcal{G}_{12}(i\omega_n)]_{jj'} = \left[\mathcal{G}^0_{12}(i\omega_n)\right]_{jj'} - |J|S\sum_\delta [\mathcal{G}_{12}(i\omega_n)]_{j\delta}\left(\left[\mathcal{G}^0_{22}(i\omega_n)\right]_{\delta j'} - \left[\mathcal{G}^0_{12}(i\omega_n)\right]_{0j'}\right) \tag{4.22}$$

$$[\mathcal{G}_{21}(i\omega_n)]_{jj'} = \left[\mathcal{G}^0_{21}(i\omega_n)\right]_{jj'} - |J|S\sum_\delta [\mathcal{G}_{22}(i\omega_n)]_{j\delta}\left(\left[\mathcal{G}^0_{21}(i\omega_n)\right]_{\delta j'} - \left[\mathcal{G}^0_{11}(i\omega_n)\right]_{0j'}\right) \tag{4.23}$$

$$[\mathcal{G}_{22}(i\omega_n)]_{jj'} = \left[\mathcal{G}^0_{22}(i\omega_n)\right]_{jj'} - |J|S\sum_\delta [\mathcal{G}_{22}(i\omega_n)]_{j\delta}\left(\left[\mathcal{G}^0_{22}(i\omega_n)\right]_{\delta j'} - \left[\mathcal{G}^0_{12}(i\omega_n)\right]_{0j'}\right). \tag{4.24}$$

To make contact with the tunneling conductance we note that in the limit $a/\lambda \ll 1$, the conductance is proportional to the integral over energy of the local dynamical structure factor. It follows that the differential conductance is proportional to the local dynamical structure factor itself which, for the square lattice antiferromagnet and honeycomb lattice ferromagnet, has the feature that the single magnon contributions come from $S^{xx} = S^{yy}$ spin components. Furthermore, these are proportional, at zero temperature, to $-(1/\pi)\text{Im}\,[\mathcal{G}_{\text{ret}}(\omega = V)]_{ii}$ where $\mathcal{G}_{\text{ret}}(\omega)$ is the retarded Green's function.

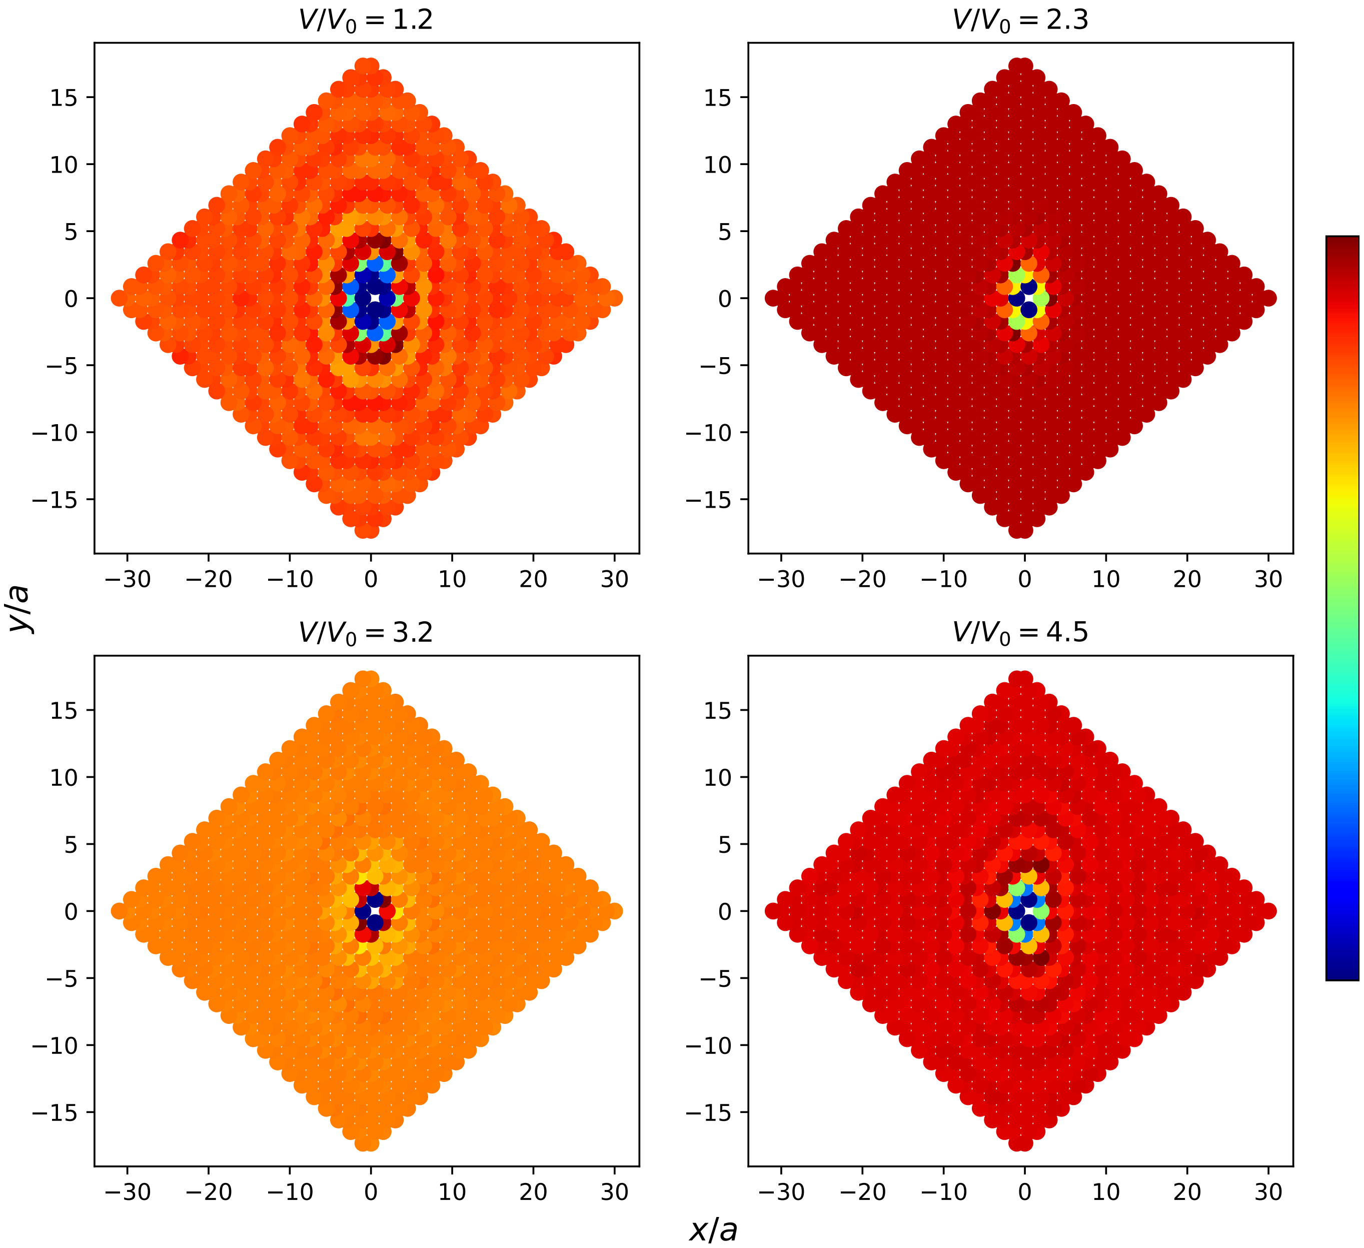


FIG. S4. Real space variation of the inelastic tunneling conductance for the Kitaev-Heisenberg model with $\theta = \frac{\pi}{2}$ and $h = 5$ on a honeycomb lattice in the presence of an impurity at the centre for a periodic 21x21 slab. The textures of the inelastic tunneling conductance around the impurity are shown on the colour scale (non-linear) at different voltage values.

### 4.2. Results

The presence of an impurity breaks the lattice translational invariance leading, in general, to finite energy textures in real space that originate from magnon scattering and interference. Examples are shown Fig. S11 for the variation of the local dynamical structure factor in the vicinity of a single vacancy site.

In this section we give more extensive magnon interference tunneling spectroscopy results than could be accommodated in the main text. We present results for the local dynamical structure factor, that is the central quantity entering into the tunneling conductance, as well as the complete differential tunneling conductance itself.

The panels in Fig. S5 exemplify the central results of the paper. These are exact calculations for the square lattice antiferromagnet with a single vacancy site. The left-hand panels show the local dynamical structure factor at constant energy for a slab with $50\times50$ magnetic primitive cells or 5000 sites but for the one A sublattice spin missing at its centre. At low energies the pattern in real space consists of circular waves emanating from the vacant site. At higher energies their wavelength becomes shorter

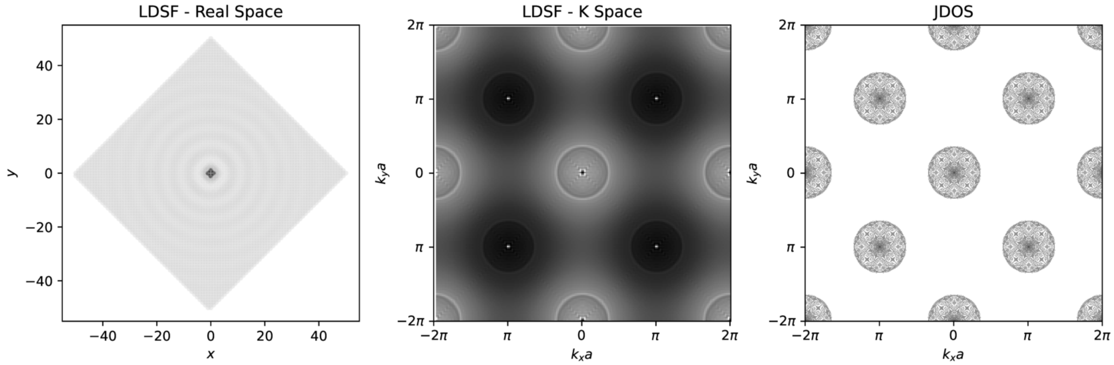


(a) $\omega/4JS = 0.375$

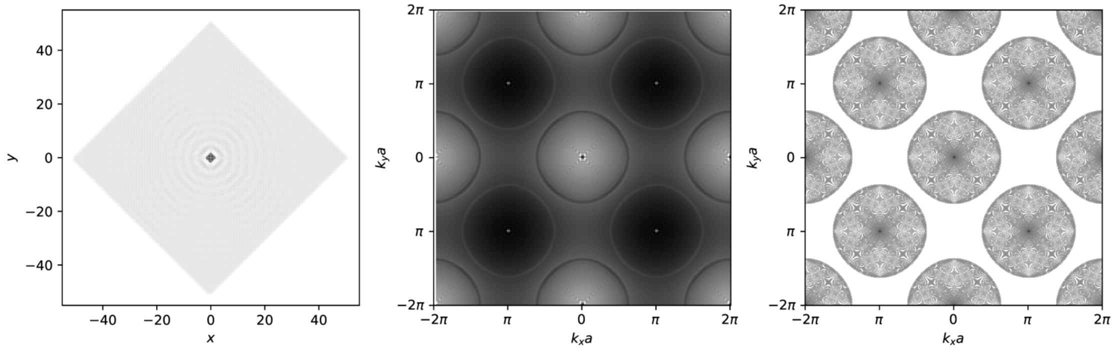


(b) $\omega/4JS = 0.625$

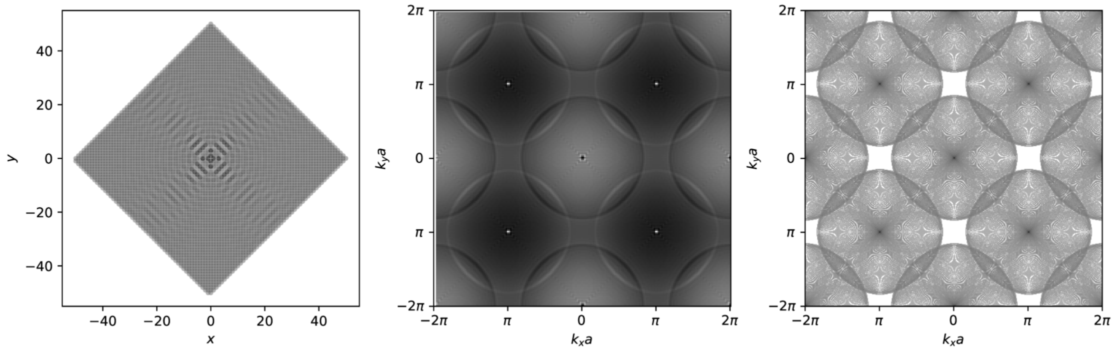


(c) $\omega/4JS = 0.775$

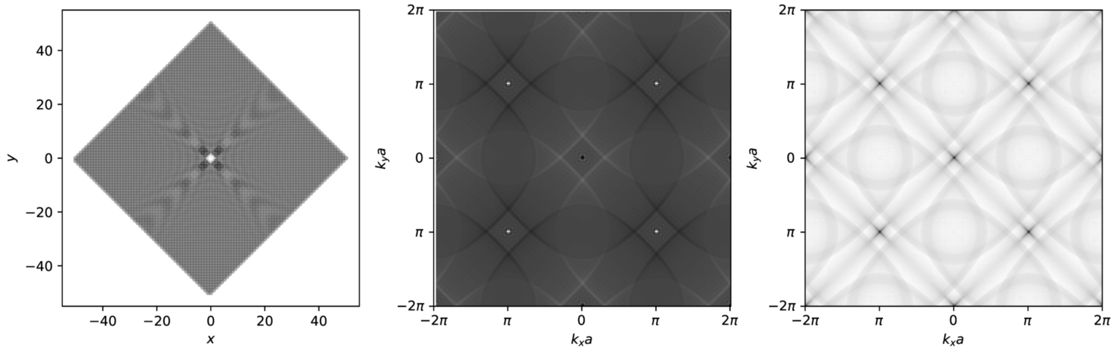


(d) $\omega/4JS = 0.975$

FIG. S5. Magnon QPI results for the square lattice Heisenberg antiferromagnet with a single vacancy. The left-hand panel is a constant energy map in real space around the impurity site of the local dynamical structure factor. The middle panel shows the Fourier transform of the pattern on the left. The right-hand panel is the join density of states (defined in the main text). From top to bottom the energies are $\omega/4JS = 0.375, 0.625, 0.775, 0.975$. The main text shows the result for $\omega/4JS = 0.875$.

and eventually the pattern becomes strongly anisotropic with waves radiating outwards along high symmetry directions. The corresponding patterns in Fourier space (central panels) may be compared directly to the joint densities of states calculated from the unperturbed spin wave band structure (right panels). In this and in all other momentum space panels, a constant background (corresponding to a $\mathbf{q} = 0$ peak) has been subtracted. The principal features of the corresponding plots are in good agreement although the relative weights somewhat differ. The band structure may therefore be extracted by refining a parametrization of the joint density of states. A straightforward application of this insight is that the wavelength of the circular waves at low energies corresponds to twice the characteristic wavevectors $2|\mathbf{k}|$ of the linearly dispersing Goldstone mode at fixed energy.

It is also illuminating to look at fixed position results as a function of energy or voltage. Fig. S11(a) shows the local dynamical structure factor at two positions: infinite distance and at sites neighboring the vacancy. Evidently the peak is shifted dramatically downward in energy close to the impurity site.

The square lattice antiferromagnet has a single magnon band but the technique can be generalized to multiband models. To illustrate this we consider the honeycomb lattice ferromagnet – a two-band model with finite energy Dirac points at the zone corners connecting the two bands. Fig. S6 shows that, once again, the exact local dynamical structure factor is in good qualitative agreement with the joint density of states.

It is useful to carry out a more direct calculation of the differential tunneling conductance to compare with the Green's function results. We do this also on a finite periodic cluster (of size $21 \times 21$) in order to benchmark the finite size calculation against the exact Green's function results. A direct comparison between the two is given in Fig. S7. The principal differences between the calculations are: (i) the numerical result is on a finite cluster, (ii) the exact result is the Green's function at fixed energy and the numerical result the differential tunneling conductance obtained from the difference of the conductance at energies differing by $\omega/J = 0.1$ or $1/60$th of the total bandwidth. Despite these differences, the results are in good agreement.

Both models considered so far have magnetic ground states that are robust to the presence of an impurity up to renormalization of the spin length. We consider one further model – the Kitaev-Heisenberg honeycomb model in the spin polarized phase. Such a phase may arise at zero applied magnetic field for certain exchange parameters [9] or at finite field. For concreteness, we consider the finite field case with a gapped magnon spectrum. This model has the feature that the ground state is destabilized around the vacancy (see Fig. S9). We have shown that the differential conductance calculated on a periodic $21 \times 21$ slab is sufficient to capture the principal features of the exact local dynamical structure factor. We therefore have confidence in a similar such calculation for the Kitaev-Heisenberg model especially at finite field. Fig. S8 shows the differential conductance results and the joint density of states for the Kitaev model at finite field showing, once again, good agreement.

Fig. S11(b) shows the local dynamical structure factor at fixed positions as a function of energy. These plots show the considerable variation from one site to another close to the impurity. The sharp peaks in the bulk band gap are the bound states described in the main text.

## 5. KITAEV-HEISENBERG MODEL AND TOPOLOGICAL MAGNON BANDS

The Kitaev-Heisenberg model, that was introduced in Section 2 2.2, can be used to study the effects of magnetic frustration and magnon band topology on the tunneling conductance. For the square lattice antiferromagnet and Heisenberg honeycomb ferromagnet, the lack of frustration means that the ground state is stable to the presence of impurities. This is not the case for the honeycomb ferromagnet in the presence of Kitaev couplings. Here the vector spin moments in the vicinity of the impurity cant away from the applied field direction. This is illustrated in the left-hand panel of Fig. S9(a) for a single vacancy on a slab with periodic boundary conditions and antiferromagnetic Kitaev couplings. The points show moments aligned with the out-of-plane magnetic field. Close to the impurity, the spin texture has slightly tilted spins whose components perpendicular to the field wind in a given sense at fixed distance from the impurity site and in opposite senses in neighbouring radial shells around the impurity. The tilt angle decays with some correlation length $\xi$ depending on the applied field (inset to Fig. S9(a)). This length scale is proportional to the inverse spin wave gap and diverges when the gap goes to zero at the finite threshold field.

The ground state on a semiperiodic slab follows a similar principle. The ground state is perturbed by the presence of the boundary with spins tilted in opposite senses depending on the distance from the boundary and the texture decays into the system exponentially. Finally, an impurity close to the boundary has a ground state where the impurity perturbs the boundary texture locally (middle and right-hand panels of Fig. S9(a)).

In principle, tunneling allows one to explore all these scenarios: (i) a single impurity in the bulk, (ii) a system with boundary with translational invariance parallel to the boundary and (iii) a single impurity at a tunable distance from the edge. We now explore the expected experimental signatures from these three cases.

*Single impurity in the bulk* – The spin wave spectrum for a single impurity on an $11 \times 11$ periodic slab is shown in Fig. S9(b, left). The bulk bands are visible extending between $E/E_0 = 1$ to 2.2 and from 3 to 5. They are slightly perturbed by the presence of the impurity. More strikingly the impurity leads to the presence of two flat in-gap states at energies of about 2.4 and 2.8. In the main text, we explain that the existence of these impurity bound states provides weak evidence for the topological nontriviality of the bulk bands. Fig. S9(c, left) illustrates the weight of the magnon wavefunction in the higher energy impurity bound state showing that the magnon wavefunction is localized around the impurity.

*Impurity close to boundary* – Considering a slab geometry with a zigzag boundary, we remove one spin at a site within a nearest neighbor distance of the boundary (Fig. S9 (middle panels)). The spectrum for this model is shown in Fig. S9(b, middle). The in-gap region is spanned by chiral surface states. The impurity modes are visible as nearly flat band that hybridize with the proximate edge states leading to small hybridization gaps and broadening the density of states (see Fig. 3 in the main text).

*Impurity site at the boundary* – The topological protection of the surface states implies that they are robust to the presence of disorder. Fig. S9(right panels) illustrates this fact for a single vacancy site. In contrast to the case described above where the vacancy lies close to the boundary, the impurity modes in this case have been entirely assimilated into renormalized chiral modes with broken translation invariance parallel to the slab.

*Tunneling Signatures of the foregoing cases* – In principle, tunneling spectroscopy provides experimental access to the surface states of two-dimensional magnets. The bulk magnon band gap can be inferred from a conductance plateau when the tip is positioned away from any impurities. By placing the tip above the sample directly above the edge and sweeping the voltage through the bulk band gap, one would observe the presence of some magnetic density of states. Here we address the question of whether additional information can be obtained about the surface state when the tunneling experiment is carried out in the presence of impurities. In particular, one would like to probe the edge state dispersion relations and the issue of whether the modes are of topological origin.

From the foregoing analysis, we have seen that the Chern magnon bands lead to localized impurity bound states. These may be detected using tunneling spectroscopy as discrete in-gap conductance jumps and provide weak evidence for topological protection. Further evidence comes from the robustness of the surface states to the presence of disorder.

By studying impurities at different distances to a boundary, the delocalization of the localized bulk impurity modes may be witnessed through the tunneling conductance. When the impurity is close to the boundary, the presence of the hybridization gap between edge modes and impurity states leads to a broadened feature in the conductance as the voltage is varied – in contrast to the sharp feature produced by the bulk impurity modes (Fig. S10(b)).

In addition, the highly spatially localized bulk impurity mode at fixed voltage becomes a spatially extended feature at the boundary. When the impurity is close to the boundary, this is in principle visible through a broadening of the Fourier transformed conductance. Because the edge state is chiral, scattering processes are highly constrained leading to a sharp $q = 0$ peak in the momentum along the boundary despite the translation symmetry breaking caused by the impurity. In other words, the joint density of states is sharply peaked in contrast to other examples we have seen in this paper where the bulk band structure offers many magnon scattering channels. The main effect of the impurity texture is to hybridize with the impurity mode giving the joint density of states a small width. The tunneling in the vicinity of the impurity and the boundary provides some evidence for a chiral mode coming from the very dearth of spatial features that one would otherwise expect near an impurity.

---


[1] J. Appelbaum, Phys. Rev. Lett. **17**, 91 (1966).
[2] P. W. Anderson, Phys. Rev. Lett. **17**, 95 (1966).
[3] M. Pustilnik and L. I. Glazman, Phys. Rev. Lett. **87**, 216601 (2001).
[4] M. Maltseva, M. Dzero, and P. Coleman, Phys. Rev. Lett. **103**, 206402 (2009).
[5] J. Fransson, O. Eriksson, and A. V. Balatsky, Phys. Rev. B **81**, 115454 (2010).
[6] J. Feldmeier, W. Natori, M. Knap, and J. Knolle, Phys. Rev. B **102**, 134423 (2020).
[7] J. R. Schrieffer and P. A. Wolff, Phys. Rev. **149**, 491 (1966).
[8] T. Holstein and H. Primakoff, Phys. Rev. **58**, 1098 (1940).
[9] P. A. McClarty, X.-Y. Dong, M. Gohlke, J. G. Rau, F. Pollmann, R. Moessner, and K. Penc, Phys. Rev. B **98**, 060404 (2018).
[10] D. G. Joshi, Phys. Rev. B **98**, 060405 (2018).
[11] A. V. Balatsky, I. Vekhter, and J.-X. Zhu, Rev. Mod. Phys. **78**, 373 (2006).

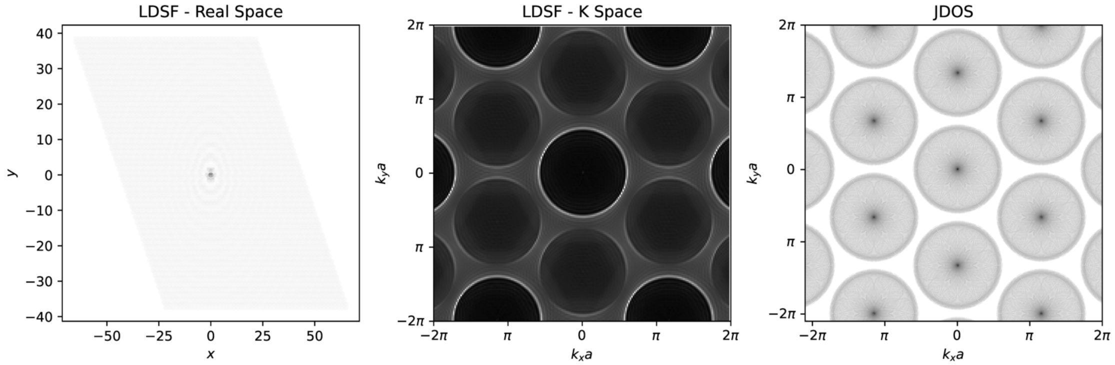


(a) $\omega/6JS = 0.1$

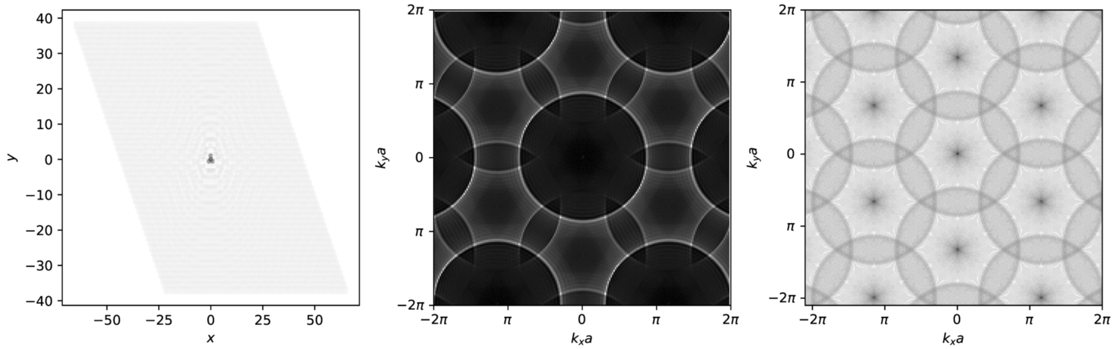

(b) $\omega/6JS = 0.2$

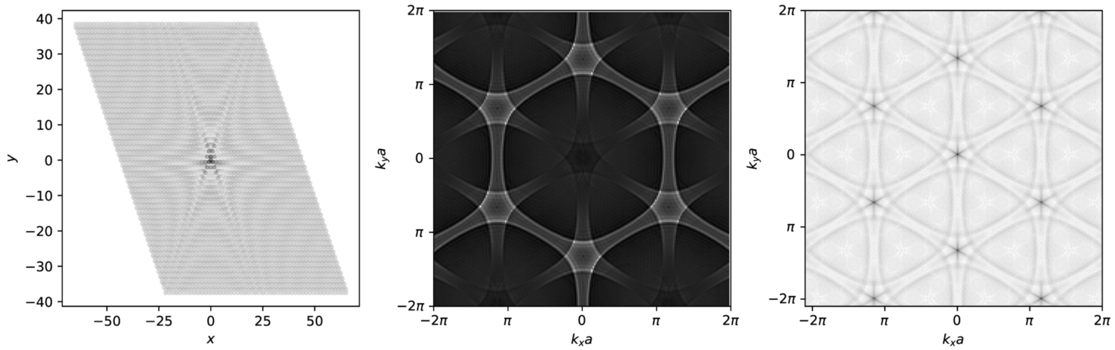

(c) $\omega/6JS = 0.3$

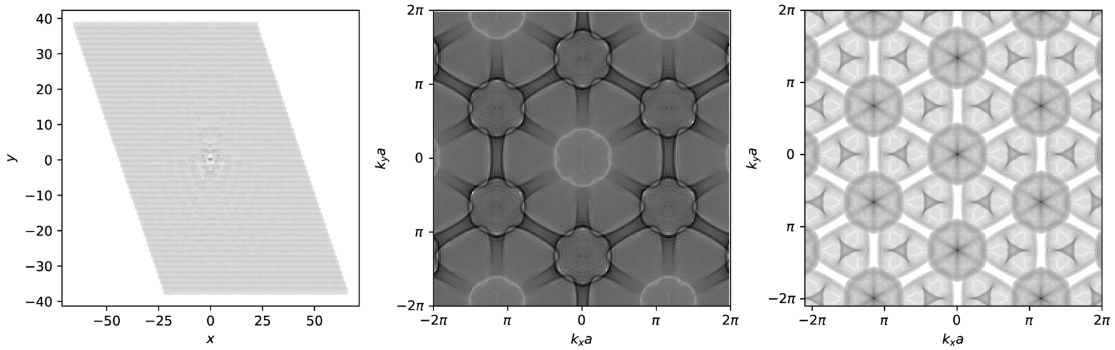

(d) $\omega/6JS = 0.367$

FIG. S6. Magnon QPI results for the honeycomb lattice Heisenberg ferromagnet with a single vacancy. The left-hand panel is a constant energy map in real space around the impurity site of the local dynamical structure factor. The middle panel shows the Fourier transform of the pattern on the left. The right-hand panel is the join density of states (defined in the main text). From top to bottom the energies are $\omega/6JS = 0.1, 0.2, 0.3$ and $0.367$. The Dirac points lie at $\omega/6JS = 0.5$.

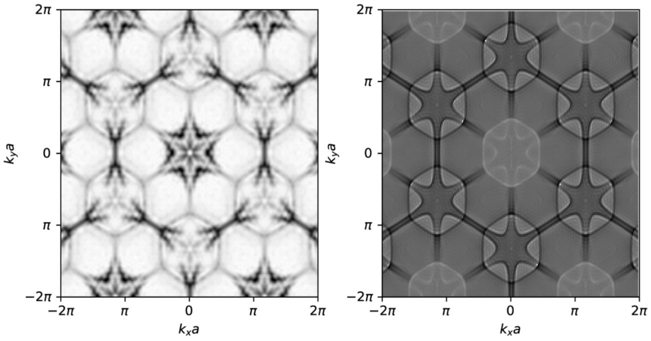


(a) $\omega/JS = 2.1$

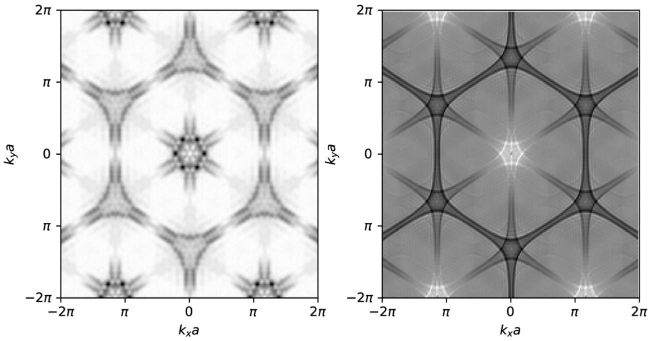


(b) $\omega/JS = 4.1$

FIG. S7. QPI plots in momentum space from the finite size differential conductance (left) and from the exact Green's function approach (right) for two different energies.

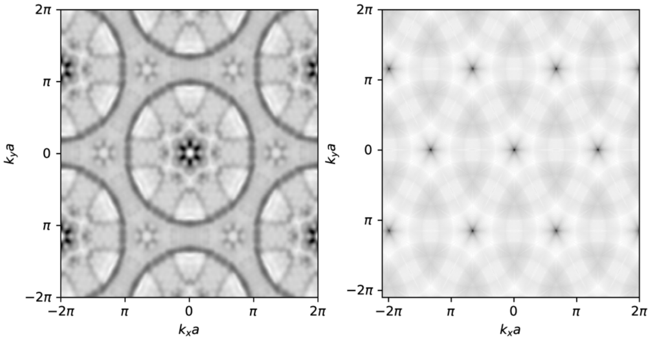


(a) $\omega/KS\,=1.6$

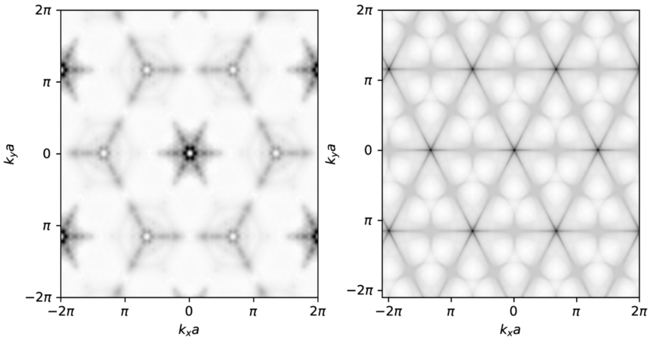


(b) $\omega/KS\,=1.9$

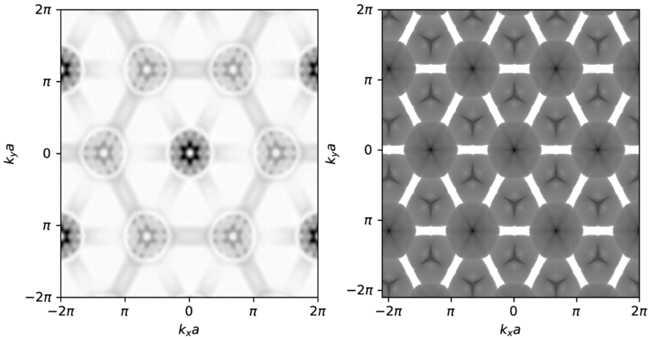


(c) $\omega/KS\,=3.2$

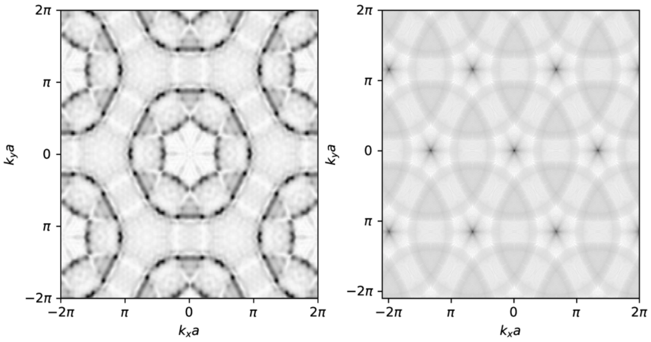


(d) $\omega/KS\,=3.8$

FIG. S8. Magnon QPI results for the honeycomb lattice Kitaev ferromagnet ($\theta = \pi/2$) with a single vacancy. The left-hand panel is the Fourier transform of the differential conductance on the periodic 21x21 slab. The right-hand panel is the joint density of states (defined in the main text). From top to bottom the energies are $\omega/KS\,=1.6, 1.9, 3.2, 3.8$ and the bands extend from 1.0 to 5.0.

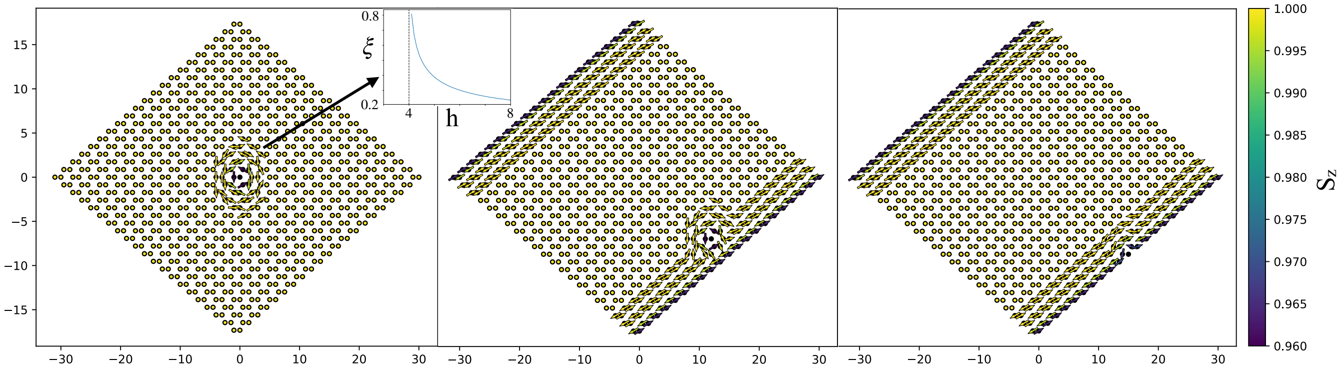


(a) Ground state

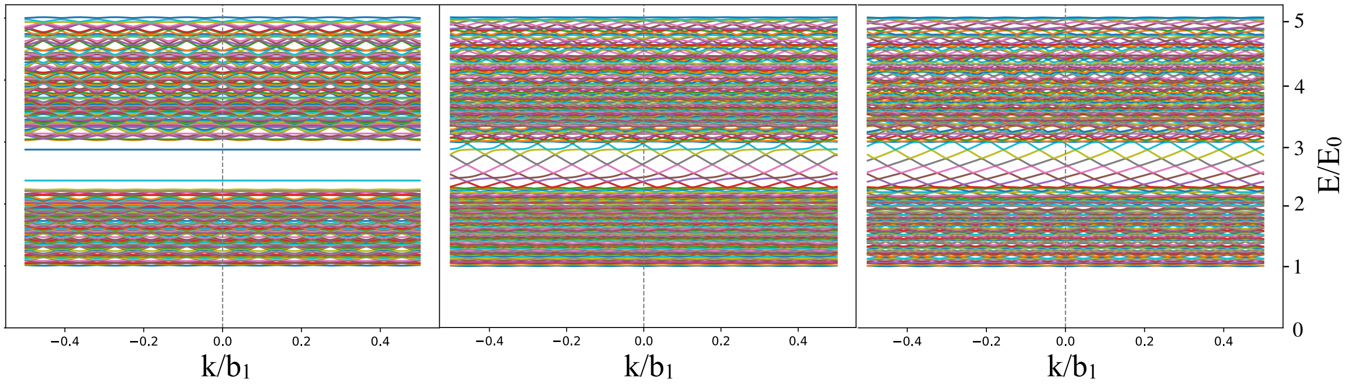


(b) Band structure

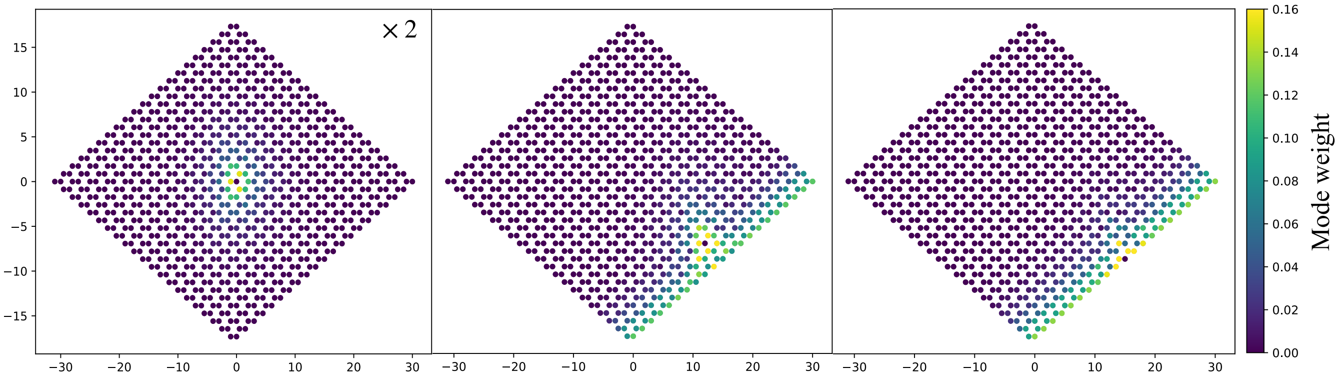


(c) Weight of local modes

FIG. S9. Calculation for the Kitaev-Heisenberg model with $\theta = \frac{\pi}{2}$ and $h = 5$ perpendicular to the plane direction on a honeycomb lattice slab periodic only in one direction. Different defects scenarios are shown: a bulk impurity (left) in a periodic slab, an impurity close to the boundary edge of a slab periodic only in one direction (center), and an impurity exactly on the boundary edge (right). a) Ground state for the three different defect scenarios in a 21x21 slab. The color shows the $S_z$ spin component and the arrow shows the transverse component direction. The defect produces a spin texture which is canted from the field direction in a vortex structure, which is counter propagating in the two different sublattices. A similar structure happens on the edges of a slab which is finite in one direction, where we can see the vortex structure connecting one edge to the other. The inset shows the spin-texture exponential decay length in unit of sublattice distance for different field direction, which diverges at $h = 4$ due to the instability of the ferromagnetic ground state. b) Bandstructure in full Brillouin Zone for a 11x11 slab. The bulk defect case on the left has a gap with two localized states (dispersionless). The defect close to the boundary hybridizes these states with the edge surface state opening up a gap (center), while when this defect is on the boundary itself produces only a renormalization (right). c) An example of $\mathbf{k} = 0$ defect mode for the different scenarios (respectively $E/E_0 = 2.88,\ 2.94,\ 2.86$), showing the local bosonic operators weights. Here we can have a real space intuition of the localization, hybridization and renormalization of the defect modes.

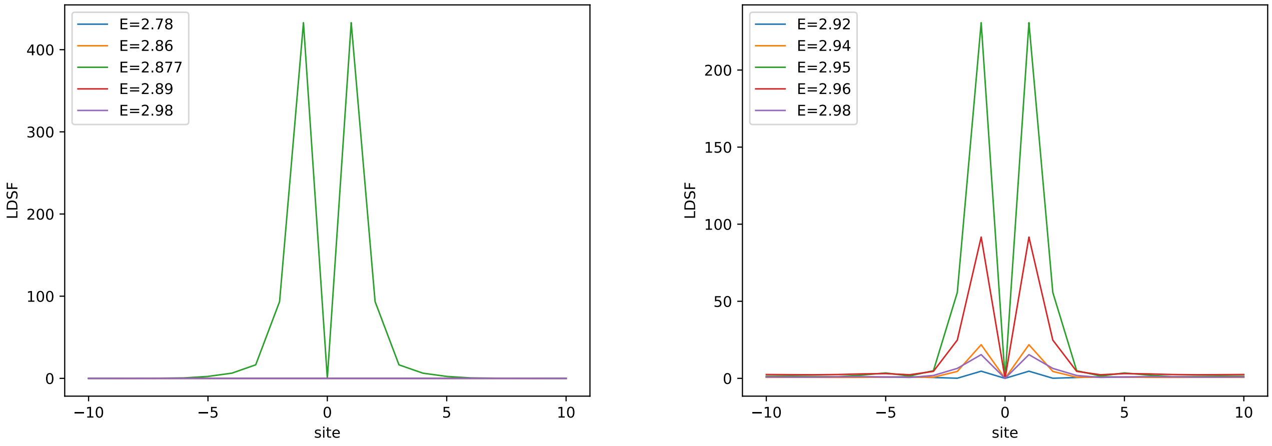


(a) Localized bulk defect

(b) Hybridized edge defect

FIG. S10. Local Dynamical Structure Factor (LDSF) for the Kitaev-Heisenberg model with $\theta = \frac{\pi}{2}$ and $h = 5$ perpendicular to the plane direction on a honeycomb lattice 21x21 slab periodic only in one direction. The x-axis are the lattice sites along the edge centered on the defect and the energy cuts are in the band gap. a) Defect in the bulk, a strong signal is present but very fine tune in energy due to the flatness of the localized state. b) Defect close to the edge producing also a strong signal. Nevertheless here, due to the hybridization with the surface state, the energy window is much larger and also small oscillations are present due to interference.

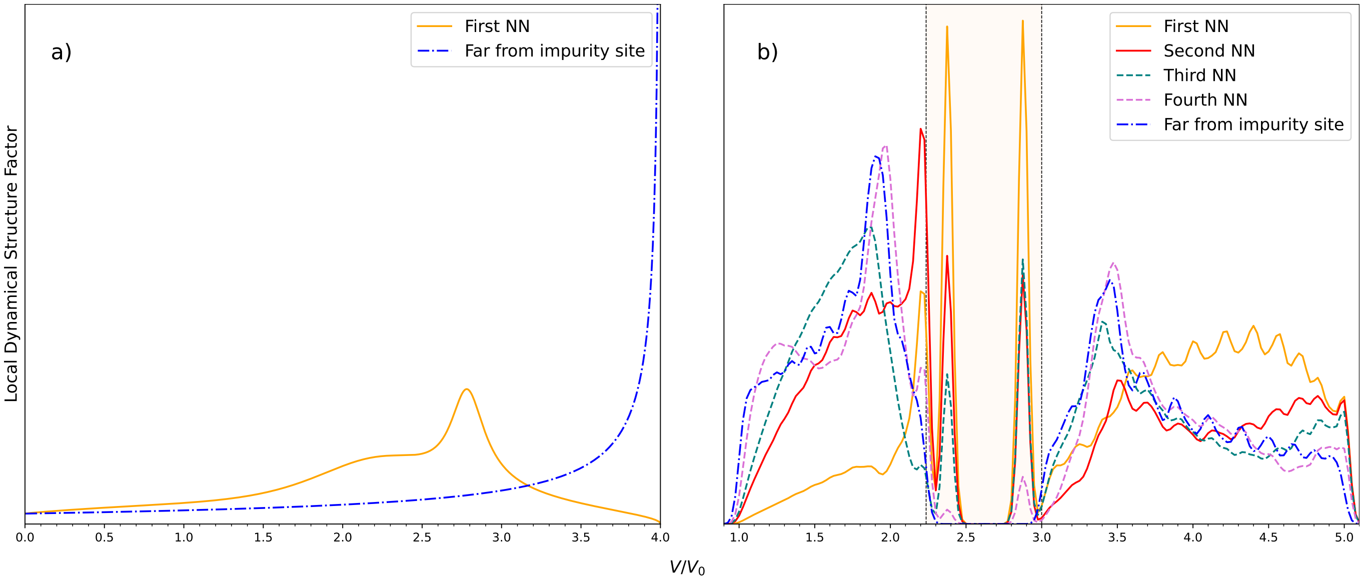


FIG. S11. (a) Local Dynamical Structure Factor (LDSF) obtained using Green's function approach for Square lattice AFM, the peak of the LDSF for the first nearest neighbor is at a considerably lower energy than the rest. (b) LDSF obtained using exact diagonalization for a $21 \times 21$ periodic slab at various distances from the impurity site obtained numerically for Kitaev-Heisenberg model for $\theta = \pi/2$ and $h = 5$ (frustrated), two distinct peaks corresponding to the impurity modes are visible within the band gap (shaded region).
